# Supplementary material for: A dependent multiplier bootstrap for the sequential empirical copula process under strong mixing
Source: arXiv:1306.3930 source file (2016-02-09)
Supplement: Supplementary file 1 [file mult-sub-supp.pdf]

Supplement to  
“A dependent multiplier bootstrap for the sequential  
empirical copula process under strong mixing”

Axel Bücher

Fakultät für Mathematik

Ruhr-Universität Bochum

44780 Bochum, Germany

`axel.buecher@ruhr-uni-bochum.de`

Ivan Kojadinovic

Laboratoire de mathématiques et applications, UMR CNRS 5142

Université de Pau et des Pays de l'Adour

B.P. 1155, 64013 Pau Cedex, France

`ivan.kojadinovic@univ-pau.fr`

October 8, 2014

## Contents

|                                                               |           |
|---------------------------------------------------------------|-----------|
| <b>C Proof of Lemma A.1</b>                                   | <b>1</b>  |
| <b>D Proof of Proposition 4.2</b>                             | <b>7</b>  |
| <b>E Proofs of Propositions 5.1 and 5.2</b>                   | <b>9</b>  |
| <b>F Bootstrap consistency based on unconditional results</b> | <b>15</b> |
| <b>G Additional simulation results</b>                        | <b>16</b> |

## C Proof of Lemma A.1

**Proof.** Fix  $m \in \{1, \dots, M\}$ . For the sake of brevity, we shall only show that the finite-dimensional distributions of  $(\tilde{\mathbb{B}}_n, \tilde{\mathbb{B}}_n^{(m)})$  converge weakly to those of  $(\mathbb{B}_C, \mathbb{B}_C^{(m)})$ , the proof

of the stated result being a more notationally complex version of the proof of the latter result.

Let  $q \in \mathbb{N}$ ,  $q > 1$ , be arbitrary, and let  $(\mathbf{u}_1, s_1, \mathbf{v}_1, t_1), \dots, (\mathbf{u}_q, s_q, \mathbf{v}_q, t_q) \in [0, 1]^{2(d+1)}$ . The result is proved if we show that

$$\begin{aligned} & \left( \tilde{\mathbb{B}}_n(s_1, \mathbf{u}_1), \tilde{\mathbb{B}}_n^{(m)}(t_1, \mathbf{v}_1), \dots, \tilde{\mathbb{B}}_n(s_q, \mathbf{u}_q), \tilde{\mathbb{B}}_n^{(m)}(t_q, \mathbf{v}_q) \right) \\ & \rightsquigarrow \left( \mathbb{B}_C(s_1, \mathbf{u}_1), \mathbb{B}_C^{(m)}(t_1, \mathbf{v}_1), \dots, \mathbb{B}_C(s_q, \mathbf{u}_q), \mathbb{B}_C^{(m)}(t_q, \mathbf{v}_q) \right). \end{aligned}$$

Let  $c_1, d_1, \dots, c_q, d_q \in \mathbb{R}$  be arbitrary. By the Cramér–Wold device, it then suffices to show that

$$Z_n = \sum_{l=1}^q c_l \tilde{\mathbb{B}}_n(s_l, \mathbf{u}_l) + \sum_{l=1}^q d_l \tilde{\mathbb{B}}_n^{(m)}(t_l, \mathbf{v}_l) \rightsquigarrow Z = \sum_{l=1}^q c_l \mathbb{B}_C(s_l, \mathbf{u}_l) + \sum_{l=1}^q d_l \mathbb{B}_C^{(m)}(t_l, \mathbf{v}_l).$$

Now, for any  $i \in \{1, \dots, n\}$ , let

$$Z_{i,n} = \sum_{l=1}^q c_l \{ \mathbf{1}(U_i \leq \mathbf{u}_l) - C(\mathbf{u}_l) \} \mathbf{1}(i \leq \lfloor ns_l \rfloor)$$

and

$$Z_{i,n}^{(m)} = \xi_{i,n}^{(m)} \sum_{l=1}^q d_l \{ \mathbf{1}(U_i \leq \mathbf{v}_l) - C(\mathbf{v}_l) \} \mathbf{1}(i \leq \lfloor nt_l \rfloor).$$

Hence,  $Z_n = n^{-1/2} \sum_{i=1}^n (Z_{i,n} + Z_{i,n}^{(m)})$ . To prove the convergence in distribution of  $Z_n$  to  $Z$ , we employ a blocking technique (see e.g. Dehling and Philipp, 2002, page 31). Each block is composed of a big subblock followed by a small subblock. Let  $0 < \eta_b < \eta_s < \varepsilon$  such that  $\eta_s < 1/2 - 1/a$ . The length of the small subblocks is  $s_n = \lfloor n^{1/2-\eta_s} \rfloor$  and the length of the big subblocks is  $b_n = \lfloor n^{1/2-\eta_b} \rfloor$  so that the length of a block is  $b_n + s_n$ . The total number of blocks is  $k_n = \lfloor n/(b_n + s_n) \rfloor$ , and we can write  $n = k_n(b_n + s_n) + \{n - k_n(b_n + s_n)\}$ . Note that  $s_n \sim n^{1/2-\eta_s}$ ,  $b_n \sim n^{1/2-\eta_b}$  and  $k_n \sim n^{1/2+\eta_b}$  and that both  $b_n$  and  $s_n$  dominate  $\ell_n$ . As we continue,  $n$  is taken sufficiently large so that  $b_n > s_n > \ell_n$ . Notice also that the condition  $\eta_s < 1/2 - 1/a$  implies that  $ns_n^{-a} \rightarrow 0$ . Now, for any  $j \in \{1, \dots, k_n\}$ , let

$$B_{j,n} = \sum_{i=(j-1)(b_n+s_n)+1}^{(j-1)(b_n+s_n)+b_n} (Z_{i,n} + Z_{i,n}^{(m)}) \quad \text{and} \quad S_{j,n} = \sum_{i=(j-1)(b_n+s_n)+b_n+1}^{j(b_n+s_n)} (Z_{i,n} + Z_{i,n}^{(m)})$$

be the sums of the  $(Z_{i,n} + Z_{i,n}^{(m)})$  in the  $j$ th big subblock and the  $j$ th small subblock, respectively. Then,

$$Z_n = n^{-1/2} \sum_{j=1}^{k_n} B_{j,n} + n^{-1/2} \sum_{j=1}^{k_n} S_{j,n} + n^{-1/2} R_n,$$

where  $R_n = \sum_{i=k_n(b_n+s_n)+1}^n (Z_{i,n} + Z_{i,n}^{(m)})$  is the sum of the  $(Z_{i,n} + Z_{i,n}^{(m)})$  after the last small subblock. It follows that

$$\begin{aligned} \text{Var}(Z_n) = & \text{Var} \left( n^{-1/2} \sum_{j=1}^{k_n} B_{j,n} \right) + 2n^{-1} \sum_{j,j'=1}^{k_n} \text{E}(B_{j,n} S_{j',n}) + 2n^{-1} \sum_{j=1}^{k_n} \text{E}(B_{j,n} R_n) \\ & + n^{-1} \sum_{j,j'=1}^{k_n} \text{E}(S_{j,n} S_{j',n}) + 2n^{-1} \sum_{j=1}^{k_n} \text{E}(S_{j,n} R_n) + \text{E}(n^{-1} R_n^2). \end{aligned} \quad (\text{C.1})$$

We shall now show that all the terms on the right except the first one tend to zero. Notice that the convergence of the fourth and sixth term to zero will imply that  $|Z_n - n^{-1/2} \sum_{j=1}^{k_n} B_{j,n}| = |n^{-1/2} \sum_{j=1}^{k_n} S_{j,n} + n^{-1/2} R_n| \xrightarrow{P} 0$ . We start with the second one. For any  $i \in \mathbb{Z}$  and any  $\mathbf{u}, \mathbf{v} \in [0, 1]^d$ , let  $\gamma(i, \mathbf{u}, \mathbf{v}) = \text{Cov}\{\mathbf{1}(U_0 \leq \mathbf{u}), \mathbf{1}(U_i \leq \mathbf{v})\}$ . We have

$$\text{E}(B_{j,n} S_{j',n}) = \sum_{i=(j-1)(b_n+s_n)+1}^{j(b_n+s_n)+b_n} \sum_{i'=(j'-1)(b_n+s_n)+b_n+1}^{j'(b_n+s_n)} \{\text{E}(Z_{i,n} Z_{i',n}) + \text{E}(Z_{i,n}^{(m)} Z_{i',n}^{(m)})\}.$$

Now,

$$|\text{E}(Z_{i,n} Z_{i',n})| \leq \sum_{l,l'=1}^q |c_l c_{l'}| |\gamma(i' - i, \mathbf{u}_l, \mathbf{u}_{l'})| \leq 4\alpha_{|i'-i|} \sum_{l,l'=1}^q |c_l c_{l'}|,$$

where the last inequality is a consequence of Lemma 3.9 in Dehling and Philipp (2002), which implies that

$$\sup_{\mathbf{u}, \mathbf{v} \in [0,1]^d} |\gamma(i, \mathbf{u}, \mathbf{v})| \leq 4\alpha_{|i|}, \quad i \in \mathbb{Z}. \quad (\text{C.2})$$

Similarly,

$$|\text{E}(Z_{i,n}^{(m)} Z_{i',n}^{(m)})| \leq \mathbf{1}(|i' - i| \leq \ell_n) 4\alpha_{|i'-i|} \sum_{l,l'=1}^q |d_l d_{l'}|$$

since, by Cauchy-Schwarz's inequality,  $\text{E}(\xi_{i,n}^{(m)} \xi_{i',n}^{(m)}) \leq \text{E}\{(\xi_{0,n}^{(m)})^2\} = 1$ . It follows that

$$|\text{E}(B_{j,n} S_{j',n})| \leq \text{const} \times \sum_{i=1}^{b_n} \sum_{i'=b_n+1}^{b_n+s_n} \alpha_{|i-i'|} \leq \text{const} \times \sum_{i=1}^{b_n+s_n-1} i\alpha_i < \infty$$

since  $\sum_{i=1}^{\infty} i\alpha_i < \infty$ . Similarly, we obtain that  $|\text{E}(B_{j,n} S_{j-1,n})| < \infty$ . For  $j' \geq j+1$  or  $j > j'+1$ ,  $\text{E}(B_{j,n} S_{j',n}) = O(b_n s_n \alpha_{b_n}) = O(b_n s_n b_n^{-a})$ . Hence,

$$2n^{-1} \sum_{j,j'=1}^{k_n} \text{E}(B_{j,n} S_{j',n}) = O(n^{-1} k_n) + O(n^{-1} k_n^2 b_n s_n b_n^{-a}) = O(b_n^{-1}) + O(n s_n b_n^{-a-1}).$$

Since  $n s_n b_n^{-a-1} < n s_n^{-a}$ , the previous term converges to zero. In a similar way, for the third summand in (C.1), we have

$$\begin{aligned} 2n^{-1} \sum_{j=1}^{k_n} \text{E}(B_{j,n} R_n) &= 2n^{-1} \sum_{j=1}^{k_n-1} \text{E}(B_{j,n} R_n) + 2n^{-1} \text{E}(B_{k_n,n} R_n) \\ &= O(n^{-1} k_n b_n (n - k_n (b_n + s_n)) \alpha_{b_n}) + O(n^{-1} b_n (n - k_n (b_n + s_n))) \\ &= O(b_n^{-a+1}) + O(n^{-1} b_n^2) \rightarrow 0 \end{aligned}$$

using the fact that  $n - k_n(b_n + s_n) < b_n + s_n$ . The case of the fifth summand is similar. Regarding the fourth summand in (C.1), we have

$$\mathbb{E}(S_{j,n}S_{j',n}) = \sum_{i=(j-1)(b_n+s_n)+b_n+1}^{j(b_n+s_n)} \sum_{i'=(j'-1)(b_n+s_n)+b_n+1}^{j'(b_n+s_n)} \{\mathbb{E}(Z_{i,n}Z_{i',n}) + \mathbb{E}(Z_{i,n}^{(m)}Z_{i',n}^{(m)})\},$$

which implies that

$$\mathbb{E}(S_{j,n}^2) \leq \text{const} \times \sum_{i,i'=b_n+1}^{b_n+s_n} \alpha_{|i'-i|} \leq \text{const} \times 2 \sum_{i=0}^{s_n-1} (s_n - i) \alpha_i \leq \text{const} \times s_n \sum_{i=0}^{\infty} \alpha_i = O(s_n)$$

and that, for  $j \neq j'$ ,  $\mathbb{E}(S_{j,n}S_{j',n}) = O(s_n^2 \alpha_{b_n}) = O(s_n^2 b_n^{-a})$ . Hence,

$$n^{-1} \sum_{j,j'=1}^{k_n} \mathbb{E}(S_{j,n}S_{j',n}) = O(n^{-1}k_n s_n) + O(n^{-1}k_n^2 s_n^2 b_n^{-a}) = O(b_n^{-1} s_n) + O(n s_n^2 b_n^{-a-2})$$

which converges to 0 since  $b_n^{-1} s_n \rightarrow 0$  and  $n s_n^2 b_n^{-a-2} < n s_n^{-a}$ . Finally, for the sixth summand in (C.1), we have

$$\mathbb{E}(n^{-1}R_n^2) = O(n^{-1}(n - k_n(b_n + s_n))^2) = O(n^{-1}(b_n + s_n)^2) = O(n^{-1}b_n^2)$$

since  $n - k_n(b_n + s_n) < b_n + s_n$ .

In order to prove that  $Z_n$  converges in distribution to  $Z$ , it suffices therefore to prove that  $n^{-1/2} \sum_{j=1}^{k_n} B_{j,n}$  converges in distribution to  $Z$ . Let  $\psi_{j,n}(t) = \exp(itn^{-1/2}B_{j,n})$ ,  $t \in \mathbb{R}$ ,  $j \in \{1, \dots, k_n\}$ , and observe that the characteristic function of  $n^{-1/2} \sum_{j=1}^{k_n} B_{j,n}$  can be written as  $t \mapsto \mathbb{E} \left\{ \prod_{j=1}^{k_n} \psi_{j,n}(t) \right\}$ . Also, for two  $\sigma$ -fields  $\mathcal{F}_1$  and  $\mathcal{F}_2$ , let

$$\alpha(\mathcal{F}_1, \mathcal{F}_2) = \sup_{A \in \mathcal{F}_1, B \in \mathcal{F}_2} |\mathbb{P}(A \cap B) - \mathbb{P}(A)\mathbb{P}(B)|.$$

Now, for any  $t \in \mathbb{R}$ , we can write

$$\begin{aligned} \left| \mathbb{E} \left\{ \prod_{j=1}^{k_n} \psi_{j,n}(t) \right\} - \prod_{j=1}^{k_n} \mathbb{E} \{ \psi_{j,n}(t) \} \right| &\leq \left| \mathbb{E} \left\{ \prod_{j=1}^{k_n} \psi_{j,n}(t) \right\} - \mathbb{E} \{ \psi_{1,n}(t) \} \mathbb{E} \left\{ \prod_{j=2}^{k_n} \psi_{j,n}(t) \right\} \right| \\ &\quad + |\mathbb{E} \{ \psi_{1,n}(t) \}| \left| \mathbb{E} \left\{ \prod_{j=2}^{k_n} \psi_{j,n}(t) \right\} - \mathbb{E} \{ \psi_{2,n}(t) \} \mathbb{E} \left\{ \prod_{j=3}^{k_n} \psi_{j,n}(t) \right\} \right| + \dots \\ &\quad \dots + \left| \prod_{j=1}^{k_n-2} \mathbb{E} \{ \psi_{j,n}(t) \} \right| \left| \mathbb{E} \left\{ \prod_{j=k_n-1}^{k_n} \psi_{j,n}(t) \right\} - \prod_{j=k_n-1}^{k_n} \mathbb{E} \{ \psi_{j,n}(t) \} \right|. \end{aligned}$$

Using the fact that the modulus of a characteristic function is smaller than one and applying  $k_n - 1$  times Lemma 3.9 of Dehling and Philipp (2002), we obtain

$$\left| \mathbb{E} \left\{ \prod_{j=1}^{k_n} \psi_{j,n}(t) \right\} - \prod_{j=1}^{k_n} \mathbb{E} \{ \psi_{j,n}(t) \} \right| \leq 2\pi k_n \max_{1 \leq i \leq k_n-1} \alpha \left[ \sigma \{ \psi_{i,n}(t) \}, \sigma \left\{ \prod_{j=i+1}^{k_n} \psi_{j,n}(t) \right\} \right].$$

Since the big subblocks are  $s_n$  observations apart, the right-hand side of the previous inequality is smaller than  $2\pi k_n \alpha_{s_n} = O(k_n s_n^{-a})$  which tends to zero as  $k_n s_n^{-a} \leq n s_n^{-a} \rightarrow 0$ . Hence, for any  $t \in \mathbb{R}$ ,

$$\left| \mathbb{E} \left\{ \prod_{j=1}^{k_n} \psi_{j,n}(t) \right\} - \prod_{j=1}^{k_n} \mathbb{E} \{ \psi_{j,n}(t) \} \right| \rightarrow 0.$$

In other words, the characteristic function of  $n^{-1/2} \sum_{j=1}^{k_n} B_{j,n}$  is asymptotically equivalent to the characteristic function of  $n^{-1/2} \sum_{j=1}^{k_n} B'_{j,n}$ , where  $B'_{1,n}, \dots, B'_{k_n,n}$  are independent and  $B'_{j,n}$  and  $B_{j,n}$  have the same distribution for all  $j \in \{1, \dots, k_n\}$ . To conclude that  $n^{-1/2} \sum_{j=1}^{k_n} B_{j,n}$  converges in distribution to  $Z$ , it suffices therefore to show that  $n^{-1/2} \sum_{j=1}^{k_n} B'_{j,n}$  converges in distribution to  $Z$ . This will be accomplished using the Lindeberg–Feller central limit theorem for triangular arrays. Hence, let us first show that  $\text{Var} \left( n^{-1/2} \sum_{j=1}^{k_n} B'_{j,n} \right) \rightarrow \text{Var}(Z)$ .

We have

$$\text{Var}(Z) = \sum_{l,l'=1}^q c_l c_{l'} (s_l \wedge s_{l'}) \sum_{i \in \mathbb{Z}} \gamma(i, \mathbf{u}_l, \mathbf{u}_{l'}) + \sum_{l,l'=1}^q d_l d_{l'} (t_l \wedge t_{l'}) \sum_{i \in \mathbb{Z}} \gamma(i, \mathbf{v}_l, \mathbf{v}_{l'}).$$

Note that, for any  $\mathbf{u}, \mathbf{v} \in [0, 1]^d$ ,  $\sum_{i \in \mathbb{Z}} \gamma(i, \mathbf{u}, \mathbf{v}) = \text{Cov}\{\mathbb{B}_C(1, \mathbf{u}), \mathbb{B}_C(1, \mathbf{v})\} < \infty$  since, from the fact that  $\gamma(i, \mathbf{v}, \mathbf{u}) = \gamma(-i, \mathbf{u}, \mathbf{v})$  and (C.2),

$$\sum_{i \in \mathbb{Z}} |\gamma(i, \mathbf{u}, \mathbf{v})| = \sum_{i=1}^{\infty} |\gamma(i, \mathbf{v}, \mathbf{u})| + |\gamma(0, \mathbf{u}, \mathbf{v})| + \sum_{i=1}^{\infty} |\gamma(i, \mathbf{u}, \mathbf{v})| \leq 1 + 8 \sum_{i=1}^{\infty} \alpha_i < \infty. \quad (\text{C.3})$$

Now, we shall first show that

$$\text{Var} \left( n^{-1/2} \sum_{j=1}^{k_n} B'_{j,n} \right) = \text{Var}(Z_n) + o(1)$$

and then that  $\text{Var}(Z_n) \rightarrow \text{Var}(Z)$ . We have

$$\begin{aligned} \text{Var} \left( n^{-1/2} \sum_{j=1}^{k_n} B'_{j,n} \right) &= n^{-1} \sum_{j=1}^{k_n} \text{Var}(B'_{j,n}) = n^{-1} \sum_{j=1}^{k_n} \text{Var}(B_{j,n}) \\ &= \text{Var} \left( n^{-1/2} \sum_{j=1}^{k_n} B_{j,n} \right) - n^{-1} \sum_{\substack{j,j'=1 \\ j \neq j'}}^{k_n} \mathbb{E}(B_{j,n} B_{j',n}). \end{aligned}$$

From (C.1), we know that  $\text{Var}(n^{-1/2} \sum_{j=1}^{k_n} B_{j,n}) = \text{Var}(Z_n) + o(1)$ . Hence, it remains to show that the double sum in the last displayed formula converges to 0. Proceeding as for the summands on the right of (C.1), we have that, for  $j \neq j'$ ,  $\mathbb{E}(B_{j,n} B_{j',n}) = O(b_n^2 \alpha_{s_n}) = O(b_n^2 s_n^{-a})$ . Hence,

$$n^{-1} \sum_{\substack{j,j'=1 \\ j \neq j'}}^{k_n} \mathbb{E}(B_{j,n} B_{j',n}) = O(n^{-1} k_n^2 b_n^2 s_n^{-a}) = O(n s_n^{-a}) \rightarrow 0.$$

Thus, it remains to show that  $\text{Var}(Z_n) \rightarrow \text{Var}(Z)$ . Now,

$$\text{Var}(Z_n) = n^{-1} \sum_{i,i'=1}^n \{E(Z_{i,n} Z_{i',n}) + E(Z_{i,n}^{(m)} Z_{i',n}^{(m)})\}.$$

It follows that

$$\begin{aligned} \text{Var}(Z_n) = & \sum_{l,l'=1}^q c_l c_{l'} n^{-1} \sum_{i=1}^{\lfloor ns_l \rfloor} \sum_{i'=1}^{\lfloor ns_{l'} \rfloor} \gamma(i' - i, \mathbf{u}_l, \mathbf{u}_{l'}) \\ & + \sum_{l,l'=1}^q d_l d_{l'} n^{-1} \sum_{i=1}^{\lfloor nt_l \rfloor} \sum_{i'=1}^{\lfloor nt_{l'} \rfloor} \varphi\{(i' - i)/\ell_n\} \gamma(i' - i, \mathbf{v}_l, \mathbf{v}_{l'}), \quad (\text{C.4}) \end{aligned}$$

where  $\varphi$  is the function appearing in Assumption (M3). Let us first deal with the second term on the right. Let  $l, l' \in \{1, \dots, q\}$  be arbitrary and suppose without loss of generality that  $t_l \leq t_{l'}$ . Then,

$$\begin{aligned} n^{-1} \sum_{i=1}^{\lfloor nt_l \rfloor} \sum_{i'=1}^{\lfloor nt_{l'} \rfloor} \varphi\{(i' - i)/\ell_n\} \gamma(i' - i, \mathbf{v}_l, \mathbf{v}_{l'}) = & n^{-1} \sum_{i=1}^{\lfloor nt_l \rfloor} \sum_{i'=1}^{\lfloor nt_l \rfloor} \varphi\{(i' - i)/\ell_n\} \gamma(i' - i, \mathbf{v}_l, \mathbf{v}_{l'}) \\ & + n^{-1} \sum_{i=1}^{\lfloor nt_l \rfloor} \sum_{i'=\lfloor nt_l \rfloor+1}^{\lfloor nt_{l'} \rfloor} \varphi\{(i' - i)/\ell_n\} \gamma(i' - i, \mathbf{v}_l, \mathbf{v}_{l'}). \quad (\text{C.5}) \end{aligned}$$

The first sum on the right-hand side is equal to

$$n^{-1} \sum_{i=-\lfloor nt_l \rfloor}^{\lfloor nt_l \rfloor} \{\lfloor nt_l \rfloor - |i|\} \varphi(i/\ell_n) \gamma(i, \mathbf{v}_l, \mathbf{v}_{l'}) = \sum_{i=-\lfloor nt_l \rfloor}^{\lfloor nt_l \rfloor} \{\lambda_n(0, t_l) - |i|/n\} \varphi(i/\ell_n) \gamma(i, \mathbf{v}_l, \mathbf{v}_{l'})$$

and converges to  $t_l \sum_{i \in \mathbb{Z}} \gamma(i, \mathbf{v}_l, \mathbf{v}_{l'})$  by Assumption (M3), (C.3) and dominated convergence. The second sum on the right-hand side of (C.5) is bounded in absolute value by  $4n^{-1} \sum_{i=1}^{\lfloor nt_{l'} \rfloor-1} i \alpha_i \rightarrow 0$ . Hence, the second term on the right of (C.4) converges to  $\sum_{l,l'=1}^q d_l d_{l'} (t_l \wedge t_{l'}) \sum_{i \in \mathbb{Z}} \gamma(i, \mathbf{v}_l, \mathbf{v}_{l'})$ . Similarly, the first term on the right of (C.4) converges to  $\sum_{l,l'=1}^q c_l c_{l'} (s_l \wedge s_{l'}) \sum_{i \in \mathbb{Z}} \gamma(i, \mathbf{u}_l, \mathbf{u}_{l'})$ . Thus,  $\text{Var}(Z_n) \rightarrow \text{Var}(Z)$ .

To be able to conclude that  $n^{-1/2} \sum_{j=1}^{k_n} B'_{j,n}$  converges in distribution to  $Z$ , it remains to prove the Lindeberg condition of the Lindeberg-Feller theorem, i.e., that, for every  $\delta > 0$ ,

$$n^{-1} \sum_{j=1}^{k_n} E\{(B'_{j,n})^2 \mathbf{1}(|B'_{j,n}| > n^{1/2} \delta)\} = n^{-1} \sum_{j=1}^{k_n} E\{B_{j,n}^2 \mathbf{1}(|B_{j,n}| > n^{1/2} \delta)\} \rightarrow 0.$$

Let  $\delta > 0$  be arbitrary. Using Hölder's inequality with  $p = 1 + \nu/2$ , where  $\nu > 0$  is to be chosen later on, and Markov's inequality, we have

$$n^{-1} \sum_{j=1}^{k_n} E\{B_{j,n}^2 \mathbf{1}(|B_{j,n}| > n^{1/2} \delta)\}$$

$$\begin{aligned}
&\leq n^{-1} \sum_{j=1}^{k_n} \{E(|B_{j,n}|^{2+\nu})\}^{2/(2+\nu)} \{P(|B_{j,n}| > n^{1/2}\delta)\}^{\nu/(2+\nu)} \\
&\leq n^{-1} \sum_{j=1}^{k_n} \{E(|B_{j,n}|^{2+\nu})\}^{2/(2+\nu)} \{P(|B_{j,n}|^{2+\nu} > n^{(2+\nu)/2}\delta^{2+\nu})\}^{\nu/(2+\nu)} \\
&\leq n^{-1} \sum_{j=1}^{k_n} \{E(|B_{j,n}|^{2+\nu})\}^{2/(2+\nu)} \{E(|B_{j,n}|^{2+\nu})\}^{\nu/(2+\nu)} (n^{1/2}\delta)^{-\nu} \\
&\leq n^{-1} \sum_{j=1}^{k_n} E(|B_{j,n}|^{2+\nu}) n^{-\nu/2} \delta^{-\nu}.
\end{aligned}$$

Now, from Minkowski's inequality,

$$\{E(|B_{j,n}|^{2+\nu})\}^{1/(2+\nu)} \leq \sum_{i=(j-1)(b_n+s_n)+1}^{(j-1)(b_n+s_n)+b_n} \left[ \{E(|Z_{i,n}|^{2+\nu})\}^{1/(2+\nu)} + \{E(|Z_{i,n}^{(m)}|^{2+\nu})\}^{1/(2+\nu)} \right] = O(b_n)$$

since, for any  $\nu > 0$ ,

$$\max_{1 \leq i \leq n} E(|Z_{i,n}|^{2+\nu}) \leq E \left( \left[ \sum_{l=1}^q |c_l| |\mathbf{1}(U_0 \leq \mathbf{u}_l) - C(\mathbf{u}_l)| \right]^{2+\nu} \right) < \infty,$$

and

$$\max_{1 \leq i \leq n} E(|Z_{i,n}^{(m)}|^{2+\nu}) \leq E \left( \left[ |\xi_{1,n}^{(m)}| \sum_{l=1}^q |d_l| |\mathbf{1}(U_0 \leq \mathbf{v}_l) - C(\mathbf{v}_l)| \right]^{2+\nu} \right) < \infty.$$

It follows that

$$n^{-1} \sum_{j=1}^{k_n} E\{B_{j,n}'^2 \mathbf{1}(|B_{j,n}'| > n^{1/2}\delta)\} = O(n^{-1} k_n b_n^{2+\nu} n^{-\nu/2}) = O(b_n^{1+\nu} n^{-\nu/2}) = O(n^{1/2-\eta_b(1+\nu)}),$$

which converges to zero for  $\nu > 1/(2\eta_b) - 1$ . ■

## D Proof of Proposition 4.2

Let us first introduce some additional notation similar to those used in Appendix B. Let  $\tilde{H}_n$  denote the empirical c.d.f. of the unobservable sample  $\mathbf{U}_1, \dots, \mathbf{U}_n$  and let  $\tilde{H}_{n,1}, \dots, \tilde{H}_{n,d}$  denote the corresponding marginal c.d.f.s. Also, for any  $j \in \{1, \dots, d\}$ , let

$$\tilde{H}_{n,j}^{-1}(u) = \inf\{v \in [0, 1] : \tilde{H}_{n,j}(v) \geq u\}, \quad u \in [0, 1],$$

and let

$$\tilde{H}_n^{-1}(\mathbf{u}) = \left( \tilde{H}_{n,1}^{-1}(u_1), \dots, \tilde{H}_{n,d}^{-1}(u_d) \right), \quad \mathbf{u} \in [0, 1]^d.$$

Finally, for any  $m \in \{1, \dots, M\}$ , let

$$\check{\mathbb{B}}_n^{(m)}(s, \mathbf{u}) = \frac{1}{\sqrt{n}} \sum_{i=1}^{\lfloor ns \rfloor} \xi_{i,n}^{(m)} \{ \mathbf{1}(\mathbf{U}_i \leq \mathbf{u}) - \tilde{H}_n(\mathbf{u}) \}, \quad (s, \mathbf{u}) \in [0, 1]^{d+1}.$$

The proof of Proposition 4.2 is based on two lemmas given after the proof.

**Proof of Proposition 4.2.** For any  $m \in \{1, \dots, M\}$  and  $(s, t, \mathbf{u}) \in \Delta \times [0, 1]^d$ , let

$$\tilde{\mathbb{C}}_n^{(m)}(s, t, \mathbf{u}) = \{ \tilde{\mathbb{B}}_n^{(m)}(t, \mathbf{u}) - \tilde{\mathbb{B}}_n^{(m)}(s, \mathbf{u}) \} - \sum_{j=1}^d \dot{C}_j(\mathbf{u}) \{ \tilde{\mathbb{B}}_n^{(m)}(t, \mathbf{u}^{(j)}) - \tilde{\mathbb{B}}_n^{(m)}(s, \mathbf{u}^{(j)}) \}.$$

From Theorem 2.1 and the continuous mapping theorem, we immediately obtain that

$$\left( \tilde{\mathbb{C}}_n, \tilde{\mathbb{C}}_n^{(1)}, \dots, \tilde{\mathbb{C}}_n^{(M)} \right) \rightsquigarrow \left( \mathbb{C}_C, \mathbb{C}_C^{(1)}, \dots, \mathbb{C}_C^{(M)} \right)$$

in  $\{\ell^\infty(\Delta \times [0, 1]^d)\}^{M+1}$ , where  $\tilde{\mathbb{C}}_n$  is defined in (3.1). Proceeding as in Segers (2012, proof of Proposition 3.2), we obtain that, for any  $m \in \{1, \dots, M\}$ ,

$$\sup_{(s, \mathbf{u}) \in [0, 1]^{d+1}} \left[ \left| \dot{C}_{j,n}(\mathbf{u}) - \dot{C}_j(\mathbf{u}) \right| \left| \tilde{\mathbb{B}}_n^{(m)}(s, \mathbf{u}) \right| \right] \xrightarrow{\mathbb{P}} 0$$

using Condition 4.1 and the fact that  $\tilde{\mathbb{B}}_n^{(m)} \rightsquigarrow \mathbb{B}_C^{(m)}$  in  $\ell^\infty([0, 1]^{d+1})$ . The desired result is finally a consequence of Corollary 3.5, Condition 4.1, and Lemmas D.1 and D.2 below. ■

**Lemma D.1.** *Under the conditions of Proposition 4.2, for any  $m \in \{1, \dots, M\}$ ,*

$$\sup_{(s, \mathbf{u}) \in [0, 1]^{d+1}} \left| \hat{\mathbb{B}}_n^{(m)}(s, \mathbf{u}) - \check{\mathbb{B}}_n^{(m)}\{s, \tilde{H}_n^{-1}(\mathbf{u})\} \right| \xrightarrow{\mathbb{P}} 0$$

where  $\hat{\mathbb{B}}_n^{(m)}$  is defined in (4.1).

**Proof.** The result is a consequence of Condition 3.3 and properties of generalized inverses, and the fact that, for any  $\nu \geq 1$ ,  $\sup_{n \geq 1} \mathbb{E}(|\xi_{0,n}^{(m)}|^\nu) < \infty$ , which implies that  $n^{-1/2} \max_{1 \leq i \leq n} |\xi_{i,n}^{(m)}| \xrightarrow{\mathbb{P}} 0$ . ■

**Lemma D.2.** *Under the conditions of Proposition 4.2, for any  $m \in \{1, \dots, M\}$ ,*

$$\sup_{(s, \mathbf{u}) \in [0, 1]^{d+1}} \left| \tilde{\mathbb{B}}_n^{(m)}(s, \mathbf{u}) - \check{\mathbb{B}}_n^{(m)}\{s, \tilde{H}_n^{-1}(\mathbf{u})\} \right| \xrightarrow{\mathbb{P}} 0.$$

where  $\tilde{\mathbb{B}}_n^{(m)}$  is defined in (2.2).

**Proof.** Let us first show that

$$J_n = \sup_{(s, \mathbf{u}) \in [0, 1]^{d+1}} \left| \tilde{\mathbb{B}}_n^{(m)}(s, \mathbf{u}) - \check{\mathbb{B}}_n^{(m)}(s, \mathbf{u}) \right| \xrightarrow{\mathbb{P}} 0.$$

Writing  $Z_{k,n} = \sum_{i=1}^k \xi_{i,n}^{(m)}$  for  $k \in \{1, \dots, n\}$ , we have  $J_n \leq K_n \times L_n$ , where

$$K_n = n^{-1} \max_{1 \leq k \leq n} |Z_{k,n}| \quad \text{and} \quad L_n = n^{1/2} \sup_{\mathbf{u} \in [0,1]^d} \left| \tilde{H}_n(\mathbf{u}) - C(\mathbf{u}) \right|.$$

Let  $\nu > 1$ . Then,

$$\begin{aligned} \mathbb{E} \left\{ \left( n^{-1} \max_{1 \leq k \leq n} |Z_{k,n}| \right)^\nu \right\} &= n^{-\nu} \mathbb{E} \left( \max_{1 \leq k \leq n} |Z_{k,n}|^\nu \right) \\ &\leq n^{-\nu} \mathbb{E} \left( \sum_{k=1}^n |Z_{k,n}|^\nu \right) \leq n^{1-\nu} \max_{1 \leq k \leq n} \mathbb{E} (|Z_{k,n}|^\nu). \end{aligned}$$

For  $\nu = 4$ , using the fact that the sequence  $(\xi_{i,n}^{(m)})_{i \in \mathbb{Z}}$  is strictly stationary and  $\ell_n$ -dependent, we obtain

$$\begin{aligned} \mathbb{E} (|Z_{k,n}|^4) &= \sum_{i_1, i_2, i_3, i_4=1}^k \mathbb{E} \left( \xi_{i_1,n}^{(m)} \xi_{i_2,n}^{(m)} \xi_{i_3,n}^{(m)} \xi_{i_4,n}^{(m)} \right) \leq 4! \sum_{1 \leq i_1 \leq i_2 \leq i_3 \leq i_4 \leq n} \left| \mathbb{E} \left( \xi_{i_1,n}^{(m)} \xi_{i_2,n}^{(m)} \xi_{i_3,n}^{(m)} \xi_{i_4,n}^{(m)} \right) \right| \\ &\leq 4! n \sum_{1 \leq i_2 \leq i_3 \leq i_4 \leq n} \left| \mathbb{E} \left( \xi_{1,n}^{(m)} \xi_{i_2,n}^{(m)} \xi_{i_3,n}^{(m)} \xi_{i_4,n}^{(m)} \right) \right| \leq 4! n \sum_{i_2=1}^{\ell_n} \sum_{i_3=i_2}^n \sum_{i_4=i_3}^{\ell_n} \left| \mathbb{E} \left( \xi_{1,n}^{(m)} \xi_{i_2,n}^{(m)} \xi_{i_3,n}^{(m)} \xi_{i_4,n}^{(m)} \right) \right|. \end{aligned}$$

From Cauchy-Swcharz's inequality,  $|\mathbb{E}(\xi_{1,n}^{(m)} \xi_{i_2,n}^{(m)} \xi_{i_3,n}^{(m)} \xi_{i_4,n}^{(m)})| \leq \mathbb{E}\{(\xi_{1,n}^{(m)})^4\}$ , and therefore  $\max_{1 \leq k \leq n} \mathbb{E} (|Z_{k,n}|^4) = O(n^2 \ell_n^2)$  since  $\sup_{n \geq 1} \mathbb{E}\{(\xi_{1,n}^{(m)})^4\} < \infty$ . It follows that

$$\mathbb{E} \left\{ \left( n^{-1} \max_{1 \leq k \leq n} |Z_{k,n}| \right)^4 \right\} = O(n^{-2\varepsilon}) \rightarrow 0,$$

which implies that  $K_n \xrightarrow{\mathbb{P}} 0$ . As  $a > 1$ , from Bücher (2014),  $L_n = O_{\mathbb{P}}(1)$ , which implies that  $J_n \xrightarrow{\mathbb{P}} 0$ .

It remains to show that

$$\sup_{(s, \mathbf{u}) \in [0,1]^{d+1}} \left| \check{\mathbb{B}}_n^{(m)}(s, \mathbf{u}) - \check{\mathbb{B}}_n^{(m)}\{s, \tilde{H}_n^{-1}(\mathbf{u})\} \right| \xrightarrow{\mathbb{P}} 0.$$

Combining Lemma A.3 with the fact that  $J_n \xrightarrow{\mathbb{P}} 0$ , we obtain that  $\check{\mathbb{B}}_n^{(m)}$  is asymptotically uniformly  $\|\cdot\|_1$ -equicontinuous in probability. The desired result finally follows from the fact that  $\sup_{u \in [0,1]} |\tilde{H}_{n,j}^{-1}(u) - u| = \sup_{u \in [0,1]} |\tilde{H}_{n,j}(u) - u| \xrightarrow{\mathbb{P}} 0$  for all  $j \in \{1, \dots, d\}$ , the latter convergence being a consequence of the fact that  $L_n = O_{\mathbb{P}}(1)$ .  $\blacksquare$

## E Proofs of Propositions 5.1 and 5.2

**Proof of Propositions 5.1.** From (C.2) and the fact that  $\alpha_r = O(r^{-a})$ ,  $a > 3$ , we have that

$$\sup_{\mathbf{u}, \mathbf{v} \in [0,1]^d} \sum_{k \in \mathbb{Z}} k^2 |\gamma(k, \mathbf{u}, \mathbf{v})| \leq 4 \sum_{k \in \mathbb{Z}} k^2 \alpha_{|k|} = 8 \sum_{k=1}^{\infty} k^2 \alpha_k < \infty.$$

Furthermore,

$$\begin{aligned} \mathbb{E}\{\tilde{\sigma}_n(\mathbf{u}, \mathbf{v})\} &= \frac{1}{n} \sum_{i,j=1}^n \varphi(|i-j|/\ell_n) \gamma(j-i, \mathbf{u}, \mathbf{v}) = \frac{1}{n} \sum_{k=-n}^n (n-|k|) \varphi(k/\ell_n) \gamma(k, \mathbf{u}, \mathbf{v}) \\ &= \sum_{k=-\ell_n}^{\ell_n} \varphi(k/\ell_n) \gamma(k, \mathbf{u}, \mathbf{v}) + s_n(\mathbf{u}, \mathbf{v}), \end{aligned}$$

where  $s_n(\mathbf{u}, \mathbf{v}) = -\frac{1}{n} \sum_{k=-\ell_n}^{\ell_n} |k| \varphi(k/\ell_n) \gamma(k, \mathbf{u}, \mathbf{v})$ . Using the fact that  $\varphi$  is bounded, we get

$$\sup_{\mathbf{u}, \mathbf{v} \in [0,1]^d} |s_n(\mathbf{u}, \mathbf{v})| \leq \frac{8}{n} \sum_{k=1}^{\infty} k \alpha_k = O(n^{-1}) = o(\ell_n^{-2}).$$

Now, from the second-order mean value theorem, for any  $n \geq 1$  and  $k \neq 0$ ,  $|k| \leq \ell_n$ , there exists  $\zeta_{k,n}$  strictly between 0 and  $k/\ell_n$  such that

$$\begin{aligned} \varphi(k/\ell_n) &= \varphi(0) + \varphi'(0)k/\ell_n + \varphi''(\zeta_{k,n})k^2/(2\ell_n^2) = 1 + \varphi''(\zeta_{k,n})k^2/(2\ell_n^2) \\ &= 1 + \varphi''(0)k^2/(2\ell_n^2) + \{\varphi''(\zeta_{k,n}) - \varphi''(0)\}k^2/(2\ell_n^2). \end{aligned}$$

Hence,

$$\sum_{k=-\ell_n}^{\ell_n} \varphi(k/\ell_n) \gamma(k, \mathbf{u}, \mathbf{v}) = \sum_{k=-\ell_n}^{\ell_n} \gamma(k, \mathbf{u}, \mathbf{v}) + \frac{\varphi''(0)}{2\ell_n^2} \sum_{k=-\ell_n}^{\ell_n} k^2 \gamma(k, \mathbf{u}, \mathbf{v}) + t_n(\mathbf{u}, \mathbf{v}),$$

where

$$t_n(\mathbf{u}, \mathbf{v}) = \frac{1}{2\ell_n^2} \sum_{k=-\ell_n}^{\ell_n} \{\varphi''(\zeta_{k,n}) - \varphi''(0)\} k^2 \gamma(k, \mathbf{u}, \mathbf{v}).$$

Furthermore,

$$2\ell_n^2 \sup_{\mathbf{u}, \mathbf{v} \in [0,1]^d} |t_n(\mathbf{u}, \mathbf{v})| \leq 8 \sum_{k=1}^{\ell_n} |\varphi''(\zeta_{k,n}) - \varphi''(0)| k^2 \alpha_k \rightarrow 0$$

by dominated convergence. Indeed, pointwise in  $k$ ,  $|\varphi''(\zeta_{k,n}) - \varphi''(0)| k^2 \alpha_k \rightarrow 0$  and, for any  $k \geq 1$ ,  $|\varphi''(\zeta_{k,n}) - \varphi''(0)| k^2 \alpha_k \leq 2 \sup_{x \in [-1,1]} |\varphi''(x)| k^2 \alpha_k$  which converges absolutely. Therefore,  $\sup_{\mathbf{u}, \mathbf{v} \in [0,1]^d} |t_n(\mathbf{u}, \mathbf{v})| = o(\ell_n^{-2})$ . The result finally follows with  $r_{n,1}(\mathbf{u}, \mathbf{v}) = s_n(\mathbf{u}, \mathbf{v}) + t_n(\mathbf{u}, \mathbf{v}) - \sum_{|k| > \ell_n} \gamma(k, \mathbf{u}, \mathbf{v})$  and the fact that

$$\ell_n^2 \sup_{\mathbf{u}, \mathbf{v} \in [0,1]^d} \left| \sum_{|k| > \ell_n} \gamma(k, \mathbf{u}, \mathbf{v}) \right| \leq 8 \ell_n^2 \sum_{k=\ell_n+1}^{\infty} \alpha_k \leq 8 \sum_{k=\ell_n+1}^{\infty} k^2 \alpha_k \rightarrow 0.$$

■

**Proof of Propositions 5.2.** The proof is based on an appropriate version of Eq. (A.1) of Künsch (1989). For any  $i \in \{1, \dots, n\}$  and  $\mathbf{u} \in [0,1]^d$ , let  $Y_i(\mathbf{u}) = \mathbf{1}(\mathbf{U}_i \leq \mathbf{u}) - C(\mathbf{u})$ .

Then, let us show that, for any  $\mathbf{u}, \mathbf{v}, \mathbf{w}, \mathbf{z} \in [0, 1]^d$  and any  $i, j, k, l \in \{0, \dots, n\}$  such that  $1 \leq i + j + k + l \leq n$ ,

$$\begin{aligned} & |\mathbb{E}\{Y_i(\mathbf{u})Y_{i+j}(\mathbf{v})Y_{i+j+k}(\mathbf{w})Y_{i+j+k+l}(\mathbf{z})\} - \mathbb{E}\{Y_i(\mathbf{u})Y_{i+j}(\mathbf{v})\}\mathbb{E}\{Y_{i+j+k}(\mathbf{w})Y_{i+j+k+l}(\mathbf{z})\} \\ & \quad - \mathbb{E}\{Y_i(\mathbf{u})Y_{i+j+k}(\mathbf{w})\}\mathbb{E}\{Y_{i+j}(\mathbf{v})Y_{i+j+k+l}(\mathbf{z})\} \\ & \quad - \mathbb{E}\{Y_i(\mathbf{u})Y_{i+j+k+l}(\mathbf{z})\}\mathbb{E}\{Y_{i+j}(\mathbf{v})Y_{i+j+k}(\mathbf{w})\}| \leq 16\alpha_{\max\{j,k,l\}}. \end{aligned} \quad (\text{E.1})$$

Fix  $\mathbf{u}, \mathbf{v}, \mathbf{w}, \mathbf{z} \in [0, 1]^d$  and  $i, j, k, l \in \{0, \dots, n\}$  such that  $1 \leq i + j + k + l \leq n$ , and let  $A, B_1, B_2$  and  $B_3$  denote the four terms appearing in the absolute value on the left of (E.1). Assume first that  $j = \max\{j, k, l\}$ . Then, using Lemma 3.9 in Dehling and Philipp (2002) as well as the facts that  $\mathbb{E}\{Y_1(\cdot)\} = 0$  and  $|Y_1(\cdot)| \leq 1$ , we obtain that  $|A| \leq 4\alpha_j$ ,  $|B_1| \leq 4\alpha_j$ ,  $|B_2| \leq 4\alpha_{j+k} \leq 4\alpha_j$  and  $|B_3| \leq 4\alpha_{j+k+l} \leq 4\alpha_j$ , which, combined with the triangle inequality, implies (E.1). Assume now that  $k = \max\{j, k, l\}$ . Then,  $|A - B_1| \leq 4\alpha_k$ ,  $|B_2| \leq 4\alpha_{j+k} \leq \alpha_k$  and  $|B_3| \leq 4\alpha_{j+k+l} \leq \alpha_k$ , and (E.1) holds. Finally, suppose that  $l = \max\{j, k, l\}$ . Then,  $|A| \leq 4\alpha_l$ ,  $|B_1| \leq 4\alpha_l$ ,  $|B_2| \leq 4\alpha_{k+l} \leq 4\alpha_l$  and  $|B_3| \leq 4\alpha_{j+k+l} \leq 4\alpha_l$  and (E.1) follows again.

Fix  $\mathbf{u}, \mathbf{v} \in [0, 1]^d$ . Starting from the expression of  $\tilde{\sigma}_n(\mathbf{u}, \mathbf{v})$ , we have that

$$\text{Var}\{\tilde{\sigma}_n(\mathbf{u}, \mathbf{v})\} = \frac{1}{n^2} \sum_{i,j,k,l=1}^n \varphi\{(i-j)/\ell_n\} \varphi\{(k-l)/\ell_n\} \text{Cov}\{Y_i(\mathbf{u})Y_j(\mathbf{v}), Y_k(\mathbf{u})Y_l(\mathbf{v})\}.$$

Let us now write

$$\begin{aligned} \text{Var}\{\tilde{\sigma}_n(\mathbf{u}, \mathbf{v})\} &= \frac{1}{n^2} \sum_{i,j,k,l=1}^n [\varphi\{(i-j)/\ell_n\} \varphi\{(k-l)/\ell_n\} \\ & \quad \times \{\gamma(k-i, \mathbf{u}, \mathbf{u})\gamma(l-j, \mathbf{v}, \mathbf{v}) + \gamma(l-i, \mathbf{u}, \mathbf{v})\gamma(k-j, \mathbf{v}, \mathbf{u})\}] + s_n(\mathbf{u}, \mathbf{v}), \end{aligned}$$

and show that  $\sup_{\mathbf{u}, \mathbf{v} \in [0, 1]^d} |s_n(\mathbf{u}, \mathbf{v})| = o(\ell_n/n)$ . Using the fact that  $\varphi$  is bounded by one, we have

$$\begin{aligned} \sup_{\mathbf{u}, \mathbf{v} \in [0, 1]^d} |s_n(\mathbf{u}, \mathbf{v})| &\leq \frac{1}{n^2} \sum_{i,j,k,l=1}^n \sup_{\mathbf{u}, \mathbf{v} \in [0, 1]^d} |\text{Cov}\{Y_i(\mathbf{u})Y_j(\mathbf{v}), Y_k(\mathbf{u})Y_l(\mathbf{v})\} \\ & \quad - \gamma(k-i, \mathbf{u}, \mathbf{u})\gamma(l-j, \mathbf{v}, \mathbf{v}) - \gamma(l-i, \mathbf{u}, \mathbf{v})\gamma(k-j, \mathbf{v}, \mathbf{u})|, \end{aligned}$$

which implies that

$$\begin{aligned} \sup_{\mathbf{u}, \mathbf{v} \in [0, 1]^d} |s_n(\mathbf{u}, \mathbf{v})| &\leq \frac{1}{n^2} \sum_{i,j,k,l=1}^n \sup_{\mathbf{u}, \mathbf{v}, \mathbf{w}, \mathbf{z} \in [0, 1]^d} |\mathbb{E}\{Y_i(\mathbf{u})Y_j(\mathbf{v})Y_k(\mathbf{w})Y_l(\mathbf{z})\} \\ & \quad - \mathbb{E}\{Y_i(\mathbf{u})Y_j(\mathbf{v})\}\mathbb{E}\{Y_k(\mathbf{w})Y_l(\mathbf{z})\} - \mathbb{E}\{Y_i(\mathbf{u})Y_k(\mathbf{w})\}\mathbb{E}\{Y_j(\mathbf{v})Y_l(\mathbf{z})\} \\ & \quad - \mathbb{E}\{Y_i(\mathbf{u})Y_l(\mathbf{z})\}\mathbb{E}\{Y_j(\mathbf{v})Y_k(\mathbf{w})\}| \\ &= \frac{4!}{n^2} \sum_{\substack{i,j,k,l=0 \\ 1 \leq i+j+k+l \leq n}}^n \sup_{\mathbf{u}, \mathbf{v}, \mathbf{w}, \mathbf{z} \in [0, 1]^d} |\mathbb{E}\{Y_i(\mathbf{u})Y_{i+j}(\mathbf{v})Y_{i+j+k}(\mathbf{w})Y_{i+j+k+l}(\mathbf{z})\} \\ & \quad - \mathbb{E}\{Y_i(\mathbf{u})Y_{i+j}(\mathbf{v})\}\mathbb{E}\{Y_{i+j+k}(\mathbf{w})Y_{i+j+k+l}(\mathbf{z})\}| \end{aligned}$$

$$\begin{aligned}
& - \mathbb{E}\{Y_i(\mathbf{u})Y_{i+j+k}(\mathbf{w})\}\mathbb{E}\{Y_{i+j}(\mathbf{v})Y_{i+j+k+l}(\mathbf{z})\} \\
& - \mathbb{E}\{Y_i(\mathbf{u})Y_{i+j+k+l}(\mathbf{z})\}\mathbb{E}\{Y_{i+j}(\mathbf{v})Y_{i+j+k}(\mathbf{w})\} \Big|.
\end{aligned}$$

Then, we obtain from (E.1),

$$\begin{aligned}
\sup_{\mathbf{u}, \mathbf{v} \in [0,1]^d} |s_n(\mathbf{u}, \mathbf{v})| & \leq \frac{4!}{n^2} \sum_{\substack{i,j,k,l=0 \\ 1 \leq i+j+k+l \leq n}}^n 16\alpha_{\max\{j,k,l\}} \leq \frac{384}{n} \sum_{\substack{j,k,l=0 \\ 1 \leq j+k+l \leq n}}^n \alpha_{\max\{j,k,l\}} \\
& \leq 3 \times \frac{384}{n} \sum_{j=1}^n \sum_{k,l=1}^j \alpha_j \leq \frac{1152}{n} \sum_{j=1}^{\infty} j^2 \alpha_j = o(\ell_n/n).
\end{aligned}$$

Hence, we have that

$$\begin{aligned}
\text{Var}\{\tilde{\sigma}_n(\mathbf{u}, \mathbf{v})\} & = \frac{1}{n^2} \sum_{i,j,k,l=1}^n \varphi\{(i-j)/\ell_n\} \varphi\{(k-l)/\ell_n\} \gamma(k-i, \mathbf{u}, \mathbf{u}) \gamma(l-j, \mathbf{v}, \mathbf{v}) \\
& + \frac{1}{n^2} \sum_{i,j,k,l=1}^n \varphi\{(i-j)/\ell_n\} \varphi\{(k-l)/\ell_n\} \gamma(l-i, \mathbf{u}, \mathbf{v}) \gamma(k-j, \mathbf{v}, \mathbf{u}) + s_n(\mathbf{u}, \mathbf{v}). \quad (\text{E.2})
\end{aligned}$$

Now, for any  $\mathbf{u}, \mathbf{v} \in [0, 1]^d$ , let

$$a_n(\mathbf{u}, \mathbf{v}) = \frac{1}{n} \sum_{p,q,r=-\infty}^{\infty} \varphi(p/\ell_n) \varphi\{(q-r)/\ell_n\} \gamma(q, \mathbf{u}, \mathbf{u}) \gamma(r-p, \mathbf{v}, \mathbf{v}).$$

Our next goal is to show that the first term on the right of (E.2) is equal to  $a_n(\mathbf{u}, \mathbf{v})$  plus a term that is  $o(\ell_n/n)$  uniformly in  $\mathbf{u}, \mathbf{v} \in [0, 1]^d$ . For any  $\mathbf{u}, \mathbf{v} \in [0, 1]^d$ , let

$$a_{i,n}(\mathbf{u}, \mathbf{v}) = \frac{1}{n} \sum_{p=1-i}^{n-i} \sum_{q=1-i}^{n-i} \sum_{r=1-i}^{n-i} \varphi(p/\ell_n) \varphi\{(q-r)/\ell_n\} \gamma(q, \mathbf{u}, \mathbf{u}) \gamma(r-p, \mathbf{v}, \mathbf{v}),$$

and notice that, by setting  $j = i + p$ ,  $k = i + q$  and  $l = i + r$ , the first term on the right of (E.2) can be written as  $n^{-1} \sum_{i=1}^n a_{i,n}(\mathbf{u}, \mathbf{v})$ . Hence, it suffices to show that

$$\sup_{\mathbf{u}, \mathbf{v} \in [0,1]^d} n^{-1} \sum_{i=1}^n |a_{i,n}(\mathbf{u}, \mathbf{v}) - a_n(\mathbf{u}, \mathbf{v})| = o(\ell_n/n).$$

For any  $i \in \{1, \dots, n\}$ , let  $A_{i,n} = \{1-i, 2-i, \dots, n-1-i, n-i\}$ , and let

$$\psi_n(p, q, r) = \varphi(p/\ell_n) \varphi\{(q-r)/\ell_n\} \alpha_{|q|} \alpha_{|r-p|}, \quad p, q, r \in \mathbb{Z}.$$

Then, using (C.2),

$$\sup_{\mathbf{u}, \mathbf{v} \in [0,1]^d} |a_{i,n}(\mathbf{u}, \mathbf{v}) - a_n(\mathbf{u}, \mathbf{v})| \leq \text{const} \times \frac{1}{n} \sum_{p,q,r} \psi_n(p, q, r),$$

where the sum on the right is over all  $p, q, r \in \mathbb{Z}$  such that at least one of the indices does not lie in  $A_{i,n}$ . Next, we can bound the right-hand side of the last display by the sum of

three sums  $B_{n,i,1} + B_{n,i,2} + B_{n,i,3}$ , where the first one is over  $p \in \mathbb{Z} \setminus A_{i,n}$  and  $q, r \in \mathbb{Z}$ , the second one over  $q \in \mathbb{Z} \setminus A_{i,n}$  and  $p, r \in \mathbb{Z}$  and the last one over  $r \in \mathbb{Z} \setminus A_{i,n}$  and  $p, q \in \mathbb{Z}$ . We shall estimate each of them individually and have to show that  $n^{-1} \sum_{i=1}^n B_{n,i,k} = o(\ell_n/n)$  for  $k \in \{1, 2, 3\}$ . Regarding  $B_{n,i,1}$ , we have

$$B_{n,i,1} \leq \frac{\text{const}}{n} \sum_{p=n-i+1}^{\infty} \sum_{q,r \in \mathbb{Z}} \psi_n(p, q, r) + \frac{\text{const}}{n} \sum_{p=-\infty}^{-i} \sum_{q,r \in \mathbb{Z}} \psi_n(p, q, r) =: B'_{n,i,1} + B''_{n,i,1}.$$

Now,  $B'_{n,i,1}$  is equal to 0 if  $n - i + 1 > \ell_n$ , that is, if  $i \leq n - \ell_n$ , and is bounded by a constant multiple of  $\{\ell_n - (n - i)\}/n \leq \ell_n/n$  for  $i > n - \ell_n$ . Similarly,  $B''_{n,i,1}$  is equal to 0 if  $i > \ell_n$  and is bounded by a constant multiple of  $\{\ell_n - i + 1\}/n \leq \ell_n/n$  for  $i \leq \ell_n$ . This implies that

$$\frac{1}{n} \sum_{i=1}^n B_{n,i,1} = \frac{1}{n} \left\{ \sum_{i=n-\ell_n+1}^n B'_{n,i,1} + \sum_{i=1}^{\ell_n} B''_{n,i,1} \right\} = O\{(\ell_n/n)^2\} = o(\ell_n/n).$$

Next, let us consider  $B_{n,i,2}$ , and, as previously, split the sum into two sums  $B'_{n,i,2} + B''_{n,i,2}$ , where the first considers the summands with  $q \geq n - i + 1$  and the second those with  $q \leq -i$ . Regarding  $B'_{n,i,2}$ , we distinguish two cases. On one hand, when  $i \leq n - 3\ell_n$ ,

$$\begin{aligned} B'_{n,i,2} &= \frac{\text{const}}{n} \sum_{q=n-i+1}^{\infty} \sum_{r=q-\ell_n}^{q+\ell_n} \sum_{p=-\ell_n}^{\ell_n} \psi_n(p, q, r) \leq \frac{\text{const}}{n} \sum_{q=3\ell_n}^{\infty} \alpha_q \sum_{r=q-\ell_n}^{q+\ell_n} \sum_{p=-\ell_n}^{\ell_n} \alpha_{|r-p|} \\ &\leq \frac{\text{const}}{n} \times \ell_n^2 \times \alpha_{\ell_n} \times \sum_{q=3\ell_n}^{\infty} \alpha_q = O(n^{-1} \ell_n^{2-a}) \times o(1) = o(\ell_n/n), \end{aligned}$$

where we used the fact that  $\varphi$  is bounded by one, the fact that  $|r-p| \geq r-p \geq q-2\ell_n \geq \ell_n$  (which implies that  $\alpha_{|r-p|} \leq \alpha_{\ell_n}$ ) and the assumption on the mixing rate. On the other hand, when  $i > n - 3\ell_n$ ,

$$B'_{n,i,2} \leq \frac{\text{const}}{n} \sum_{q=1}^{\infty} \alpha_q \sum_{r=q-\ell_n}^{q+\ell_n} \sum_{p=-\infty}^{\infty} \alpha_{|r-p|} = O(\ell_n/n).$$

Therefore,

$$\frac{1}{n} \sum_{i=1}^n B'_{n,i,2} = \frac{n - 3\ell_n}{n} o(\ell_n/n) + \frac{3\ell_n}{n} O(\ell_n/n) = o(\ell_n/n).$$

The quantity  $B''_{n,i,2}$  can be treated similarly. It remains therefore to consider  $B_{n,i,3}$  which we split again into two sums  $B'_{n,i,3} + B''_{n,i,3}$ , where the first considers the summands with  $r \geq n - i + 1$  and the second those with  $r \leq -i$ . On one hand, when  $i \leq n - 2\ell_n + 1$ ,

$$B'_{n,i,3} = \frac{\text{const}}{n} \sum_{r=n-i+1}^{\infty} \sum_{q=r-\ell_n}^{r+\ell_n} \sum_{p=-\ell_n}^{\ell_n} \psi_n(p, q, r) \leq \frac{\text{const}}{n} \times \alpha_{\ell_n} \times \ell_n \times \sum_{r=n-i+1}^{\infty} \sum_{p=-\ell_n}^{\ell_n} \alpha_{r-p},$$

where we used the fact that  $|q| \geq q \geq r - \ell_n \geq \ell_n$ . The double sum on the right-hand side can be bounded by  $(2\ell_n + 1) \sum_{s=\ell_n}^{\infty} \alpha_s = o(\ell_n)$ , whence  $B'_{n,i,3} = o(\ell_n/n)$  by similar

arguments as before. On the other hand, when  $i > n - 2\ell_n + 1$ ,

$$B'_{n,i,3} \leq \frac{\text{const}}{n} \sum_{r=1}^{\infty} \sum_{q \in \mathbb{Z}} \alpha_{|q|} \sum_{p=-\ell_n}^{\ell_n} \alpha_{|r-p|} = O(\ell_n/n).$$

Hence,

$$\frac{1}{n} \sum_{i=1}^n B'_{n,i,3} = \frac{n - 2\ell_n + 1}{n} o(\ell_n/n) + \frac{2\ell_n - 1}{n} O(\ell_n/n) = o(\ell_n/n),$$

The quantity  $B''_{n,i,3}$  can be treated similarly, by considering the cases  $i \geq 2\ell_n$  and  $i < 2\ell_n$ .

This completes the proof for the first term on the right (E.2). Proceeding similarly for the second term, we obtain that

$$\begin{aligned} \text{Var}\{\tilde{\sigma}_n(\mathbf{u}, \mathbf{v})\} &= \frac{1}{n} \sum_{p,q,r=-\infty}^{\infty} \varphi(p/\ell_n) \varphi\{(q-r)/\ell_n\} \gamma(q, \mathbf{u}, \mathbf{u}) \gamma(r-p, \mathbf{v}, \mathbf{v}) \\ &\quad + \frac{1}{n} \sum_{p,q,r=-\infty}^{\infty} \varphi(p/\ell_n) \varphi\{(q-r)/\ell_n\} \gamma(q, \mathbf{u}, \mathbf{v}) \gamma(r-p, \mathbf{v}, \mathbf{u}) + s'_n(\mathbf{u}, \mathbf{v}), \end{aligned}$$

where  $\sup_{\mathbf{u}, \mathbf{v} \in [0,1]^d} s'_n(\mathbf{u}, \mathbf{v}) = o(\ell_n/n)$ . Setting  $s = p - r$ , we get

$$\begin{aligned} \text{Var}\{\tilde{\sigma}_n(\mathbf{u}, \mathbf{v})\} &= \frac{1}{n} \sum_{s,q,r=-\infty}^{\infty} \varphi\{(s+r)/\ell_n\} \varphi\{(q-r)/\ell_n\} \{ \gamma(q, \mathbf{u}, \mathbf{u}) \gamma(s, \mathbf{v}, \mathbf{v}) \\ &\quad + \gamma(q, \mathbf{u}, \mathbf{v}) \gamma(s, \mathbf{u}, \mathbf{v}) \} + s'_n(\mathbf{u}, \mathbf{v}). \end{aligned}$$

To finish the proof, it remains to show that  $\sup_{\mathbf{u}, \mathbf{v} \in [0,1]^d} |s''_n(\mathbf{u}, \mathbf{v})| = o(\ell_n/n)$ , where

$$\begin{aligned} s''_n(\mathbf{u}, \mathbf{v}) &= \frac{1}{n} \sum_{s,q,r=-\infty}^{\infty} [\varphi\{(s+r)/\ell_n\} \varphi\{(q-r)/\ell_n\} - \{\varphi(r/\ell_n)\}^2] \{ \gamma(q, \mathbf{u}, \mathbf{u}) \gamma(s, \mathbf{v}, \mathbf{v}) \\ &\quad + \gamma(q, \mathbf{u}, \mathbf{v}) \gamma(s, \mathbf{u}, \mathbf{v}) \}. \end{aligned}$$

Using (C.2), we have

$$\sup_{\mathbf{u}, \mathbf{v} \in [0,1]^2} |s''_n(\mathbf{u}, \mathbf{v})| \leq \frac{\text{const}}{n} \sum_{s,q=-\infty}^{\infty} \alpha_{|q|} \alpha_{|s|} \sum_{r=-\infty}^{\infty} |\varphi\{(s+r)/\ell_n\} \varphi\{(q-r)/\ell_n\} - \{\varphi(r/\ell_n)\}^2|.$$

The sum over  $r$  on the right-hand side consists of at most  $3 \times (2\ell_n + 1)$  non-zero summands (those  $r$  for which either  $|s+r|$ ,  $|q-r|$  or  $|r|$  is smaller than or equal to  $\ell_n$ ). Now, for any  $s, q, r$  such that  $|s+r|$ ,  $|q-r|$  or  $|r|$  is smaller than or equal to  $\ell_n$ , we have, from the conditions on  $\varphi$ ,

$$\begin{aligned} &|\varphi\{(s+r)/\ell_n\} \varphi\{(q-r)/\ell_n\} - \{\varphi(r/\ell_n)\}^2| \\ &= |\varphi\{(s+r)/\ell_n\} [\varphi\{(q-r)/\ell_n\} - \varphi(r/\ell_n)] + \varphi(r/\ell_n) [\varphi\{(s+r)/\ell_n\} - \varphi(r/\ell_n)]| \\ &\leq \sup_{x \in [-1,1]} |\varphi(x)| \times [|\varphi\{(q-r)/\ell_n\} - \varphi(r/\ell_n)| + |\varphi\{(s+r)/\ell_n\} - \varphi(r/\ell_n)|] \end{aligned}$$

$$\leq \lambda(|q| + |s|)/\ell_n,$$

and therefore, from the conditions on the strongly mixing coefficients,

$$\begin{aligned} & \sum_{s,q=-\infty}^{\infty} \alpha_{|q|} \alpha_{|s|} \sum_{r=-\infty}^{\infty} |\varphi\{(s+r)/\ell_n\} \varphi\{(q-r)/\ell_n\} - \{\varphi(r/\ell_n)\}^2| \\ & \leq \sum_{s,q=-\infty}^{\infty} \alpha_{|q|} \alpha_{|s|} (6\ell_n + 3) \lambda\{|q| + |s|\}/\ell_n \leq \text{const} \sum_{s,q=-\infty}^{\infty} \alpha_{|q|} \alpha_{|s|} \{|q| + |s|\} < \infty. \end{aligned}$$

Hence,  $\sup_{\mathbf{u}, \mathbf{v} \in [0,1]^2} |s_n''(\mathbf{u}, \mathbf{v})| = O(1/n) = o(\ell_n/n)$ . The stated result finally follows from the fact that  $\ell_n^{-1} \sum_{r=-\ell_n}^{\ell_n} \{\varphi(r/\ell_n)\}^2 = \int_{-1}^1 \varphi(x)^2 dx + o(1)$ .  $\blacksquare$

## F Bootstrap consistency based on unconditional results

In this section, we state a rather general result showing that unconditional results such as those given in Theorem 2.1, Corollary 2.2 or Proposition 4.2 are sufficient for showing bootstrap consistency in many situations of practical interest. Roughly speaking, once unconditional results for empirical processes such as those mentioned above are transferred to the real line (typically by means of the continuous mapping theorem or the functional delta method), Proposition F.1 below shows that, the larger the sample size and the number of bootstrap replicates, the more meaningful it is to estimate a quantile of the statistic of interest by the corresponding empirical quantile of the bootstrap sample.

**Proposition F.1.** *For any integer  $M \geq 1$ , assume that there exists random variables  $S_n, S_n^{(1)}, \dots, S_n^{(M)}$  such that*

$$(S_n, S_n^{(1)}, \dots, S_n^{(M)}) \rightsquigarrow (S, S^{(1)}, \dots, S^{(M)}),$$

where  $S$ , the weak limit of  $S_n$ , is a continuous random variable, and  $S^{(1)}, \dots, S^{(M)}$  are independent copies of  $S$ . Furthermore, let  $K_{n,M}$  be the empirical c.d.f. computed from  $S_n^{(1)}, \dots, S_n^{(M)}$  and, for all  $y \in (0, 1]$ , let  $K_{n,M}^{-1}(y) = \inf\{x \in \mathbb{R} : K_{n,M}(x) \geq y\}$ . Then, for any  $\alpha \in (0, 1)$ ,

$$\lim_{M \rightarrow \infty} \lim_{n \rightarrow \infty} \mathbb{P}\{S_n \geq K_{n,M}^{-1}(1 - \alpha)\} = \alpha. \quad (\text{F.1})$$

*Proof.* The proof is almost identical to the proof of Corollary 3.7 in Bücher et al. (2014).

Fix  $\alpha \in (0, 1)$  and assume first that  $\alpha \notin \mathbb{Q}$ . Using the right continuity of  $K_{n,M}$ , we have that, for all  $x \in \mathbb{R}$ ,  $x \geq K_{n,M}^{-1}(1 - \alpha)$  if and only if  $K_{n,M}(x) \geq 1 - \alpha$ , and therefore

$$\mathbb{P}\{S_n \geq K_{n,M}^{-1}(1 - \alpha)\} = \mathbb{P}\{K_{n,M}(S_n) \geq 1 - \alpha\}.$$

Let  $K_M$  be the empirical c.d.f. computed from  $S^{(1)}, \dots, S^{(M)}$  and let us first show that, for any fixed integer  $M \geq 1$ , we have

$$\lim_{n \rightarrow \infty} \mathbb{P}\{K_{n,M}(S_n) \geq 1 - \alpha\} = \mathbb{P}\{K_M(S) \geq 1 - \alpha\}. \quad (\text{F.2})$$

For that purpose, consider the map  $\Psi : \mathbb{R}^{M+1} \rightarrow \mathbb{R}$  by  $\Psi(t_0, \dots, t_M) = M^{-1} \sum_{m=1}^M \mathbf{1}(t_m \leq t_0)$  and note that  $\Psi$  is continuous at any point  $(t_0, \dots, t_M) \in \mathbb{R}^{M+1}$  such that  $t_0 \neq t_i$  for all  $i \in \{1, \dots, M\}$ . Then, since  $(S_n, S_n^{(1)}, \dots, S_n^{(M)}) \rightsquigarrow (S, S^{(1)}, \dots, S^{(M)})$  with the limit having pairwise different coordinates almost surely, the continuous mapping theorem implies that  $K_{n,M}(S_n) \rightsquigarrow K_M(S)$  as  $n \rightarrow \infty$ . Since  $\alpha \notin \{1/M, \dots, M/M\}$  and  $P\{K_M(S) = 1 - \alpha\} = 0$ , the portmanteau lemma implies (F.2).

In order to prove the desired result, it remains to show that

$$\lim_{M \rightarrow \infty} P\{K_M(S) \geq 1 - \alpha\} = \alpha. \quad (\text{F.3})$$

Fix  $0 < \varepsilon < 1 - \alpha$ . By the Glivenko–Cantelli lemma, we may choose an integer  $M_0 = M_0(\varepsilon) \geq 1$  such that, for any  $M \geq M_0$ ,

$$P\left\{\sup_{x \in \mathbb{R}} |K_M(x) - K(x)| > \varepsilon\right\} \leq \varepsilon,$$

where  $K$  denotes the c.d.f. of  $S$ . For all such  $M$ ,

$$\begin{aligned} P\{K_M(S) \geq 1 - \alpha\} &= P\{K_M(S) - K(S) + K(S) \geq 1 - \alpha\} \\ &\leq P\{K_M(S) - K(S) \geq \varepsilon\} + P\{K(S) \geq 1 - \alpha - \varepsilon\} \leq \varepsilon + \alpha + \varepsilon = \alpha + 2\varepsilon. \end{aligned}$$

Furthermore,

$$P\{K_M(S) \geq 1 - \alpha\} \geq P\{K(S) \geq 1 - \alpha + \varepsilon\} = \alpha - \varepsilon.$$

Thus,  $|P\{K_M(S) \geq 1 - \alpha\} - \alpha| \leq 2\varepsilon$ . This proves (F.3), and together with (F.2), we obtain that (F.1) holds for any  $\alpha \in (0, 1) \cap (\mathbb{R} \setminus \mathbb{Q})$ .

Following van der Vaart (1998, proof of Lemma 23.3), one can extend (F.1) to the case  $\alpha \in \mathbb{Q}$  using the fact that  $\alpha \mapsto P\{S_n \geq K_{n,M}^{-1}(1 - \alpha)\}$  is a monotone function of  $\alpha$  as well as the right hand side of (F.1), which is also continuous.  $\blacksquare$

## G Additional simulation results

This section contains additional simulation results. The general setting is described in Section 6 of the paper. We only report the results when  $C$  is the Gumbel–Hougaard copula with parameter 1.5, the results for the three other copulas being qualitatively similar.

### G.1 Analogues of Figure 2 for other values of $p$

This subsection contains analogues of Figure 2 for other values of the quantile order  $p$ . The statistic is still  $S_n$  and the legend is the same as in Figure 2.

### G.1.1 Statistic $S_n$ , $p = 0.25$

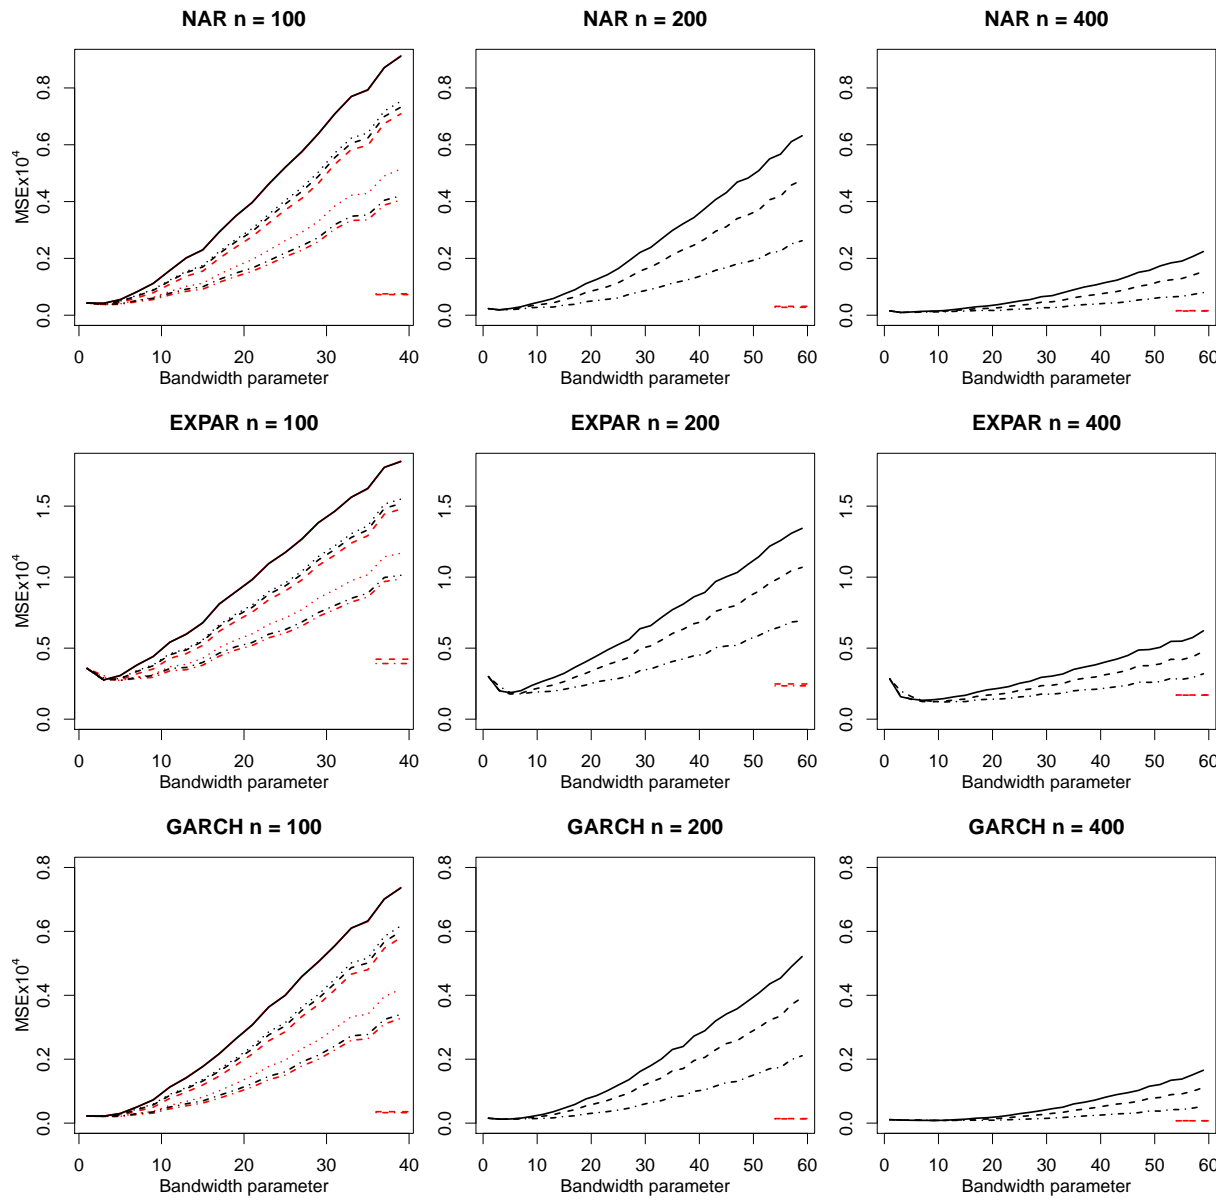

### G.1.2 Statistic $S_n$ , $p = 0.5$

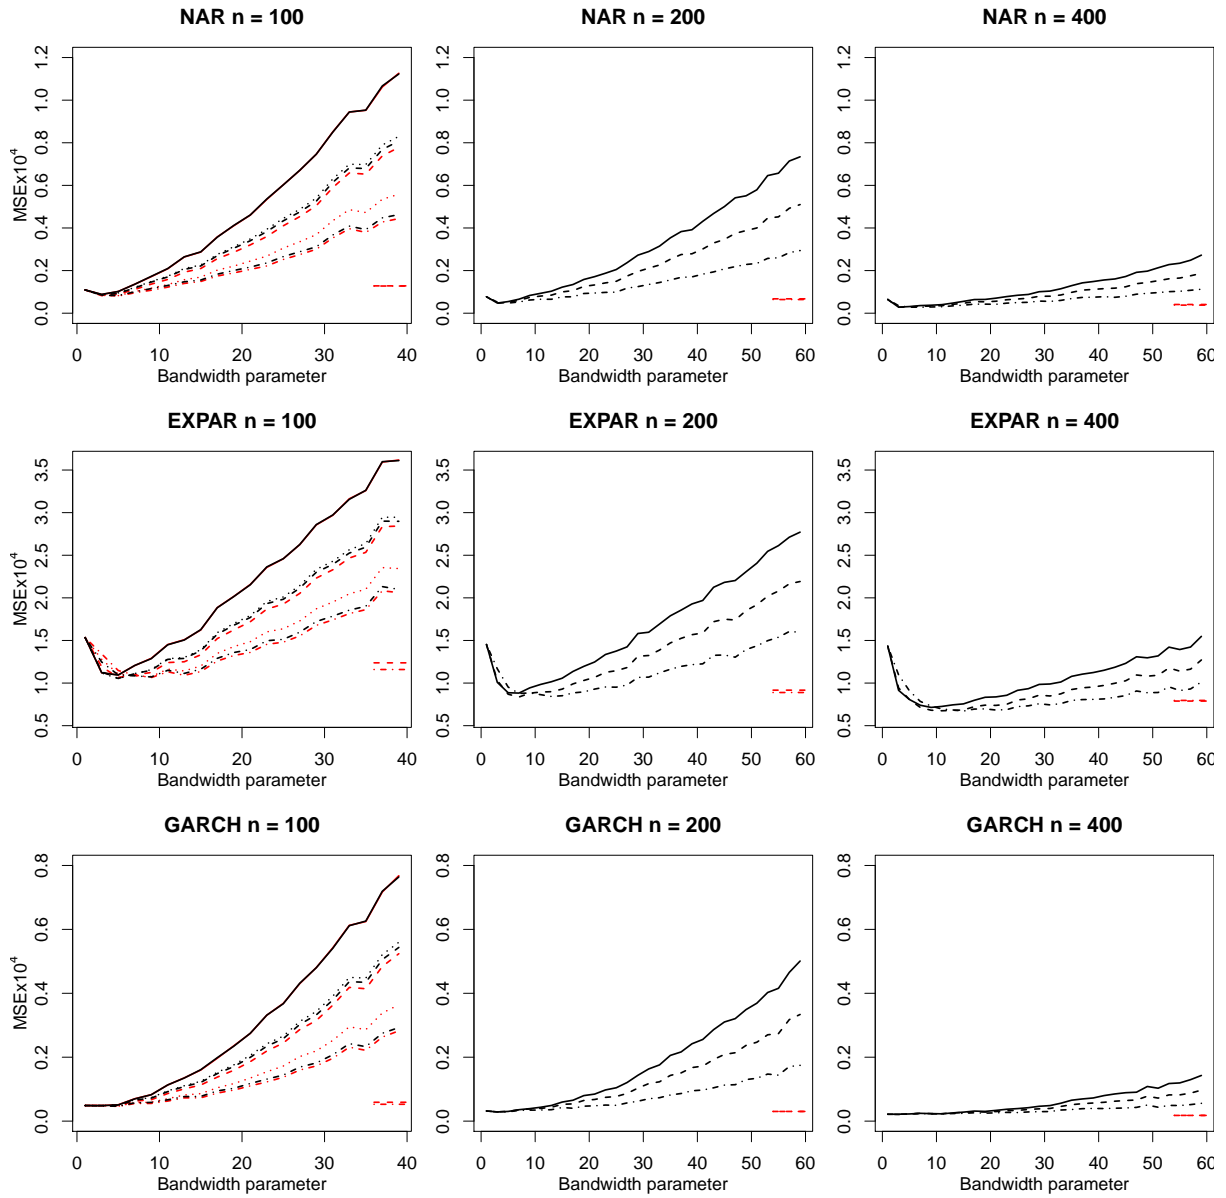

### G.1.3 Statistic $S_n$ , $p = 0.75$

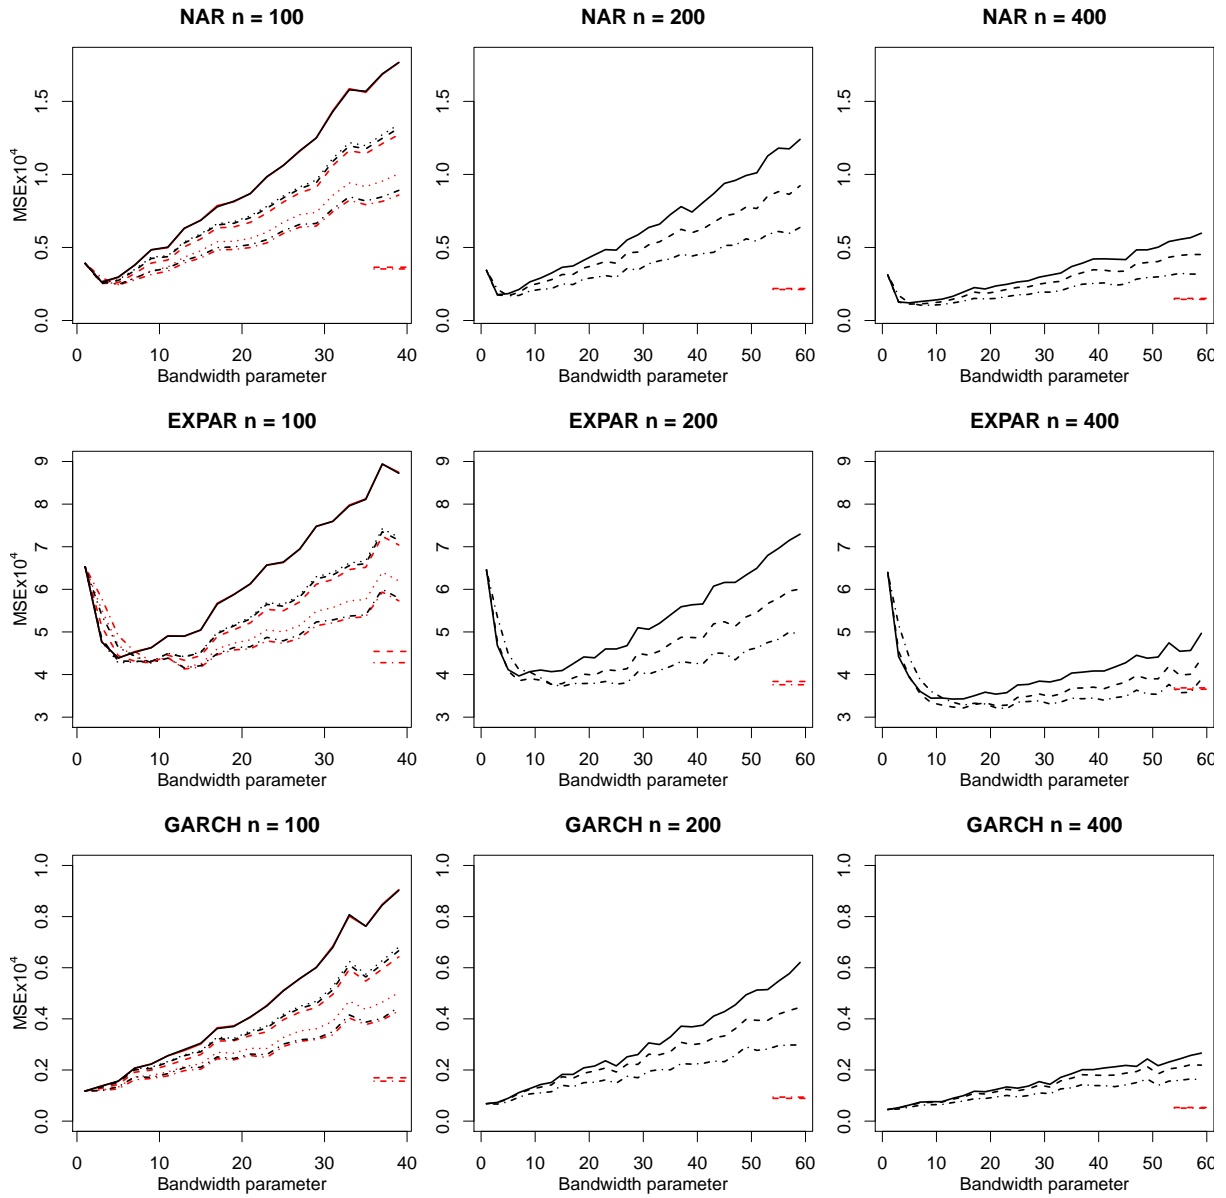

### G.1.4 Statistic $S_n$ , $p = 0.90$

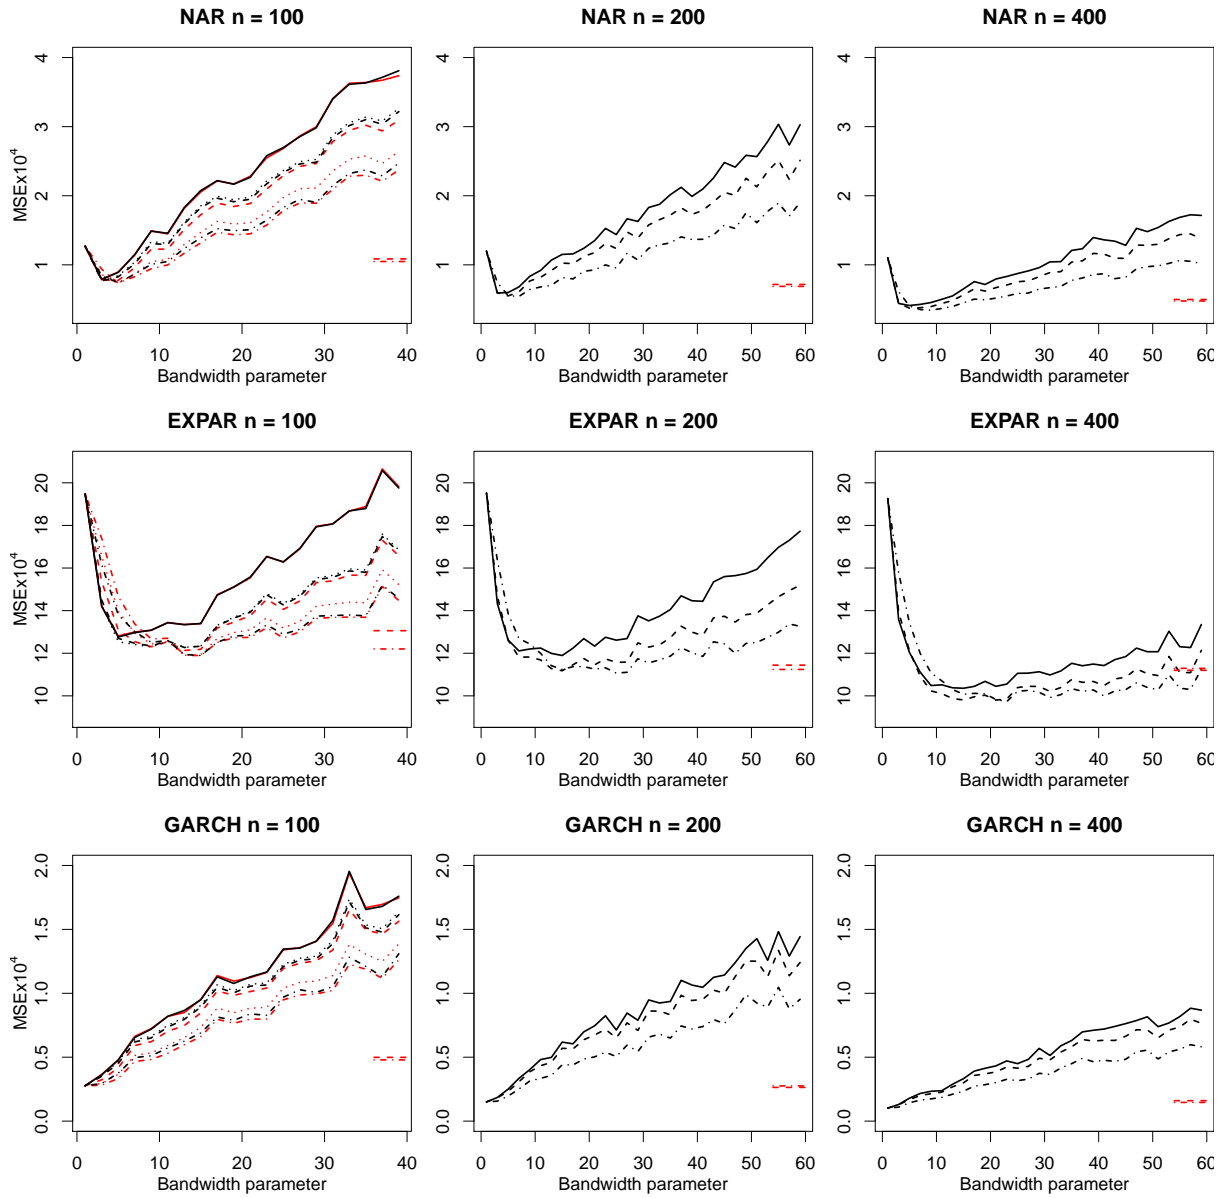

### G.1.5 Statistic $S_n$ , $p = 0.99$

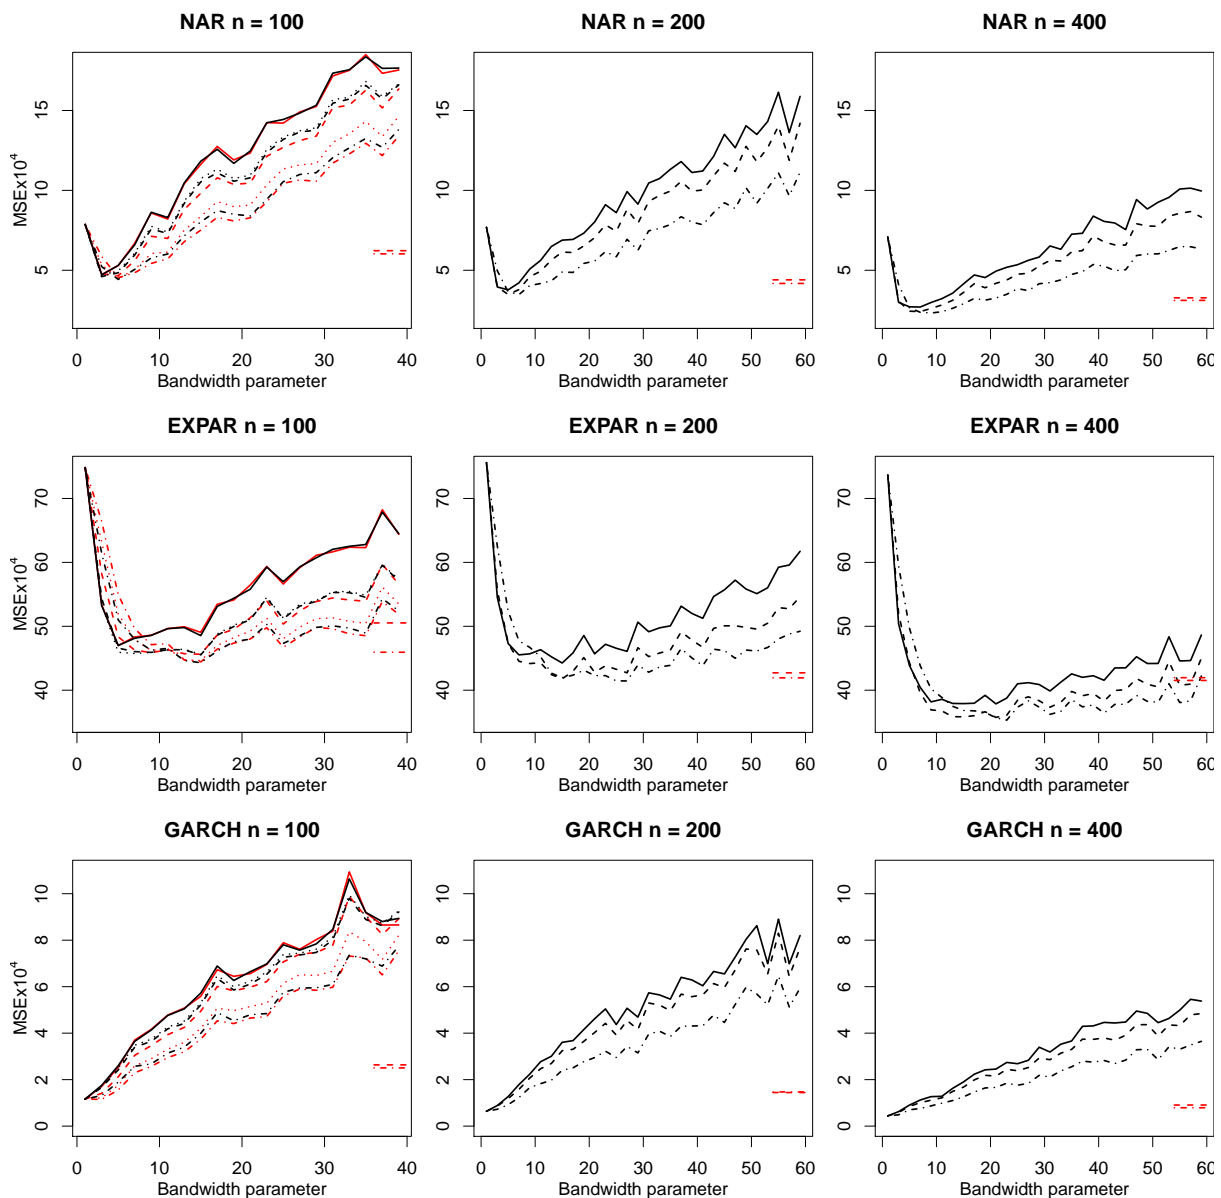

## G.2 Analogues of Figure 2 for the statistic $T_n$

This subsection contains analogues of Figure 2 for the statistic  $T_n$ . The legend is the same as in Figure 2.

## G.2.1 Statistic $T_n$ , $p = 0.25$

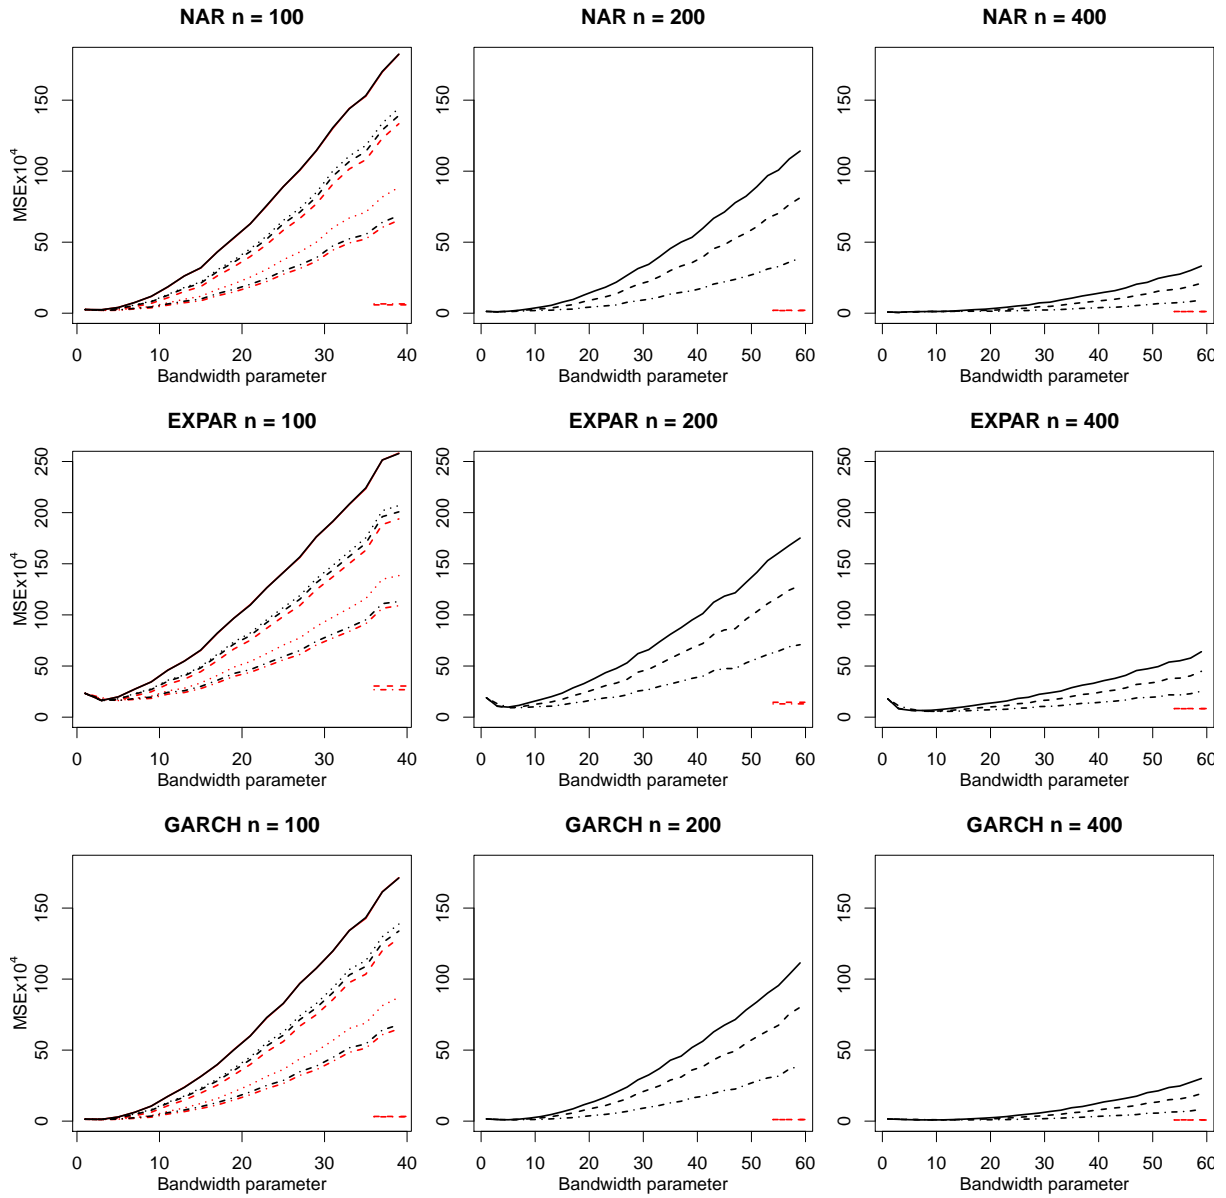

## G.2.2 Statistic $T_n$ , $p = 0.5$

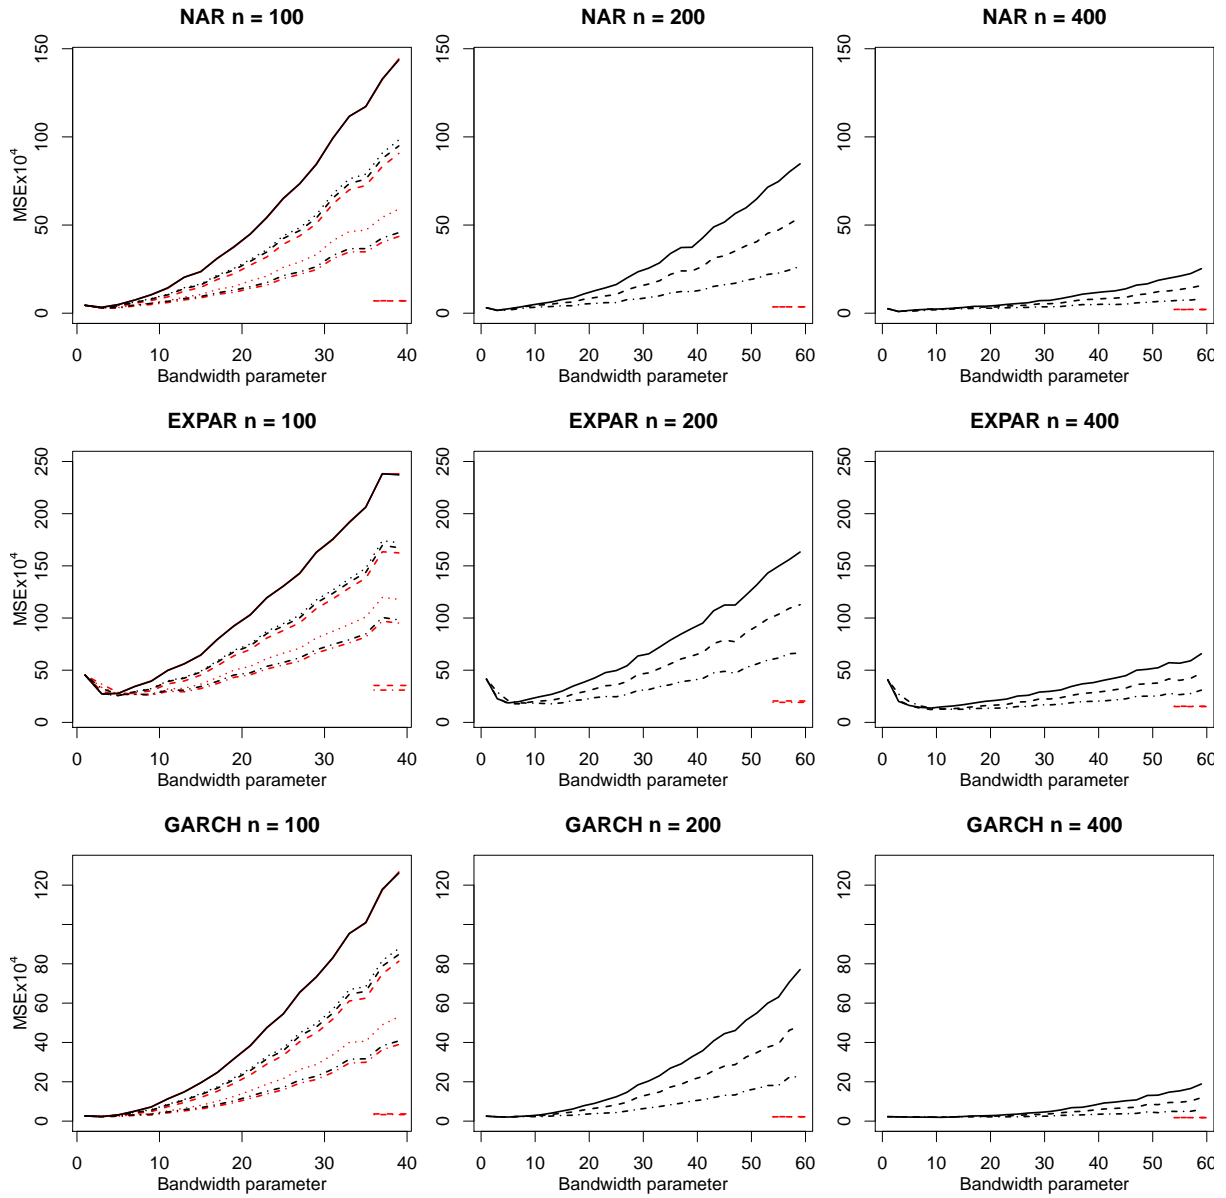

### G.2.3 Statistic $T_n$ , $p = 0.75$

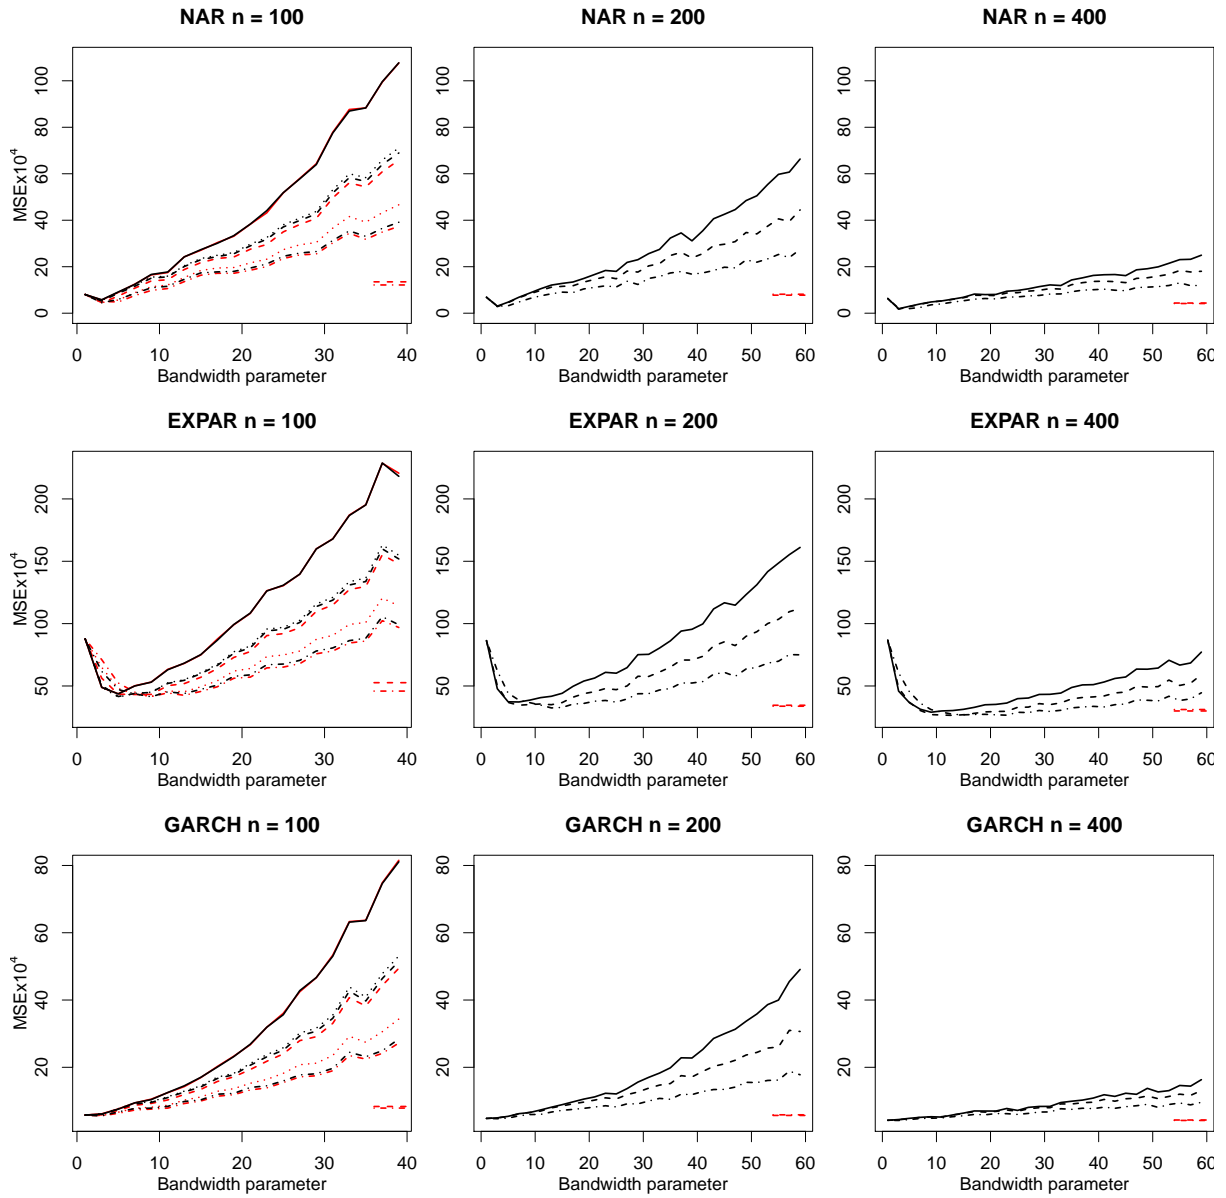

## G.2.4 Statistic $T_n$ , $p = 0.90$

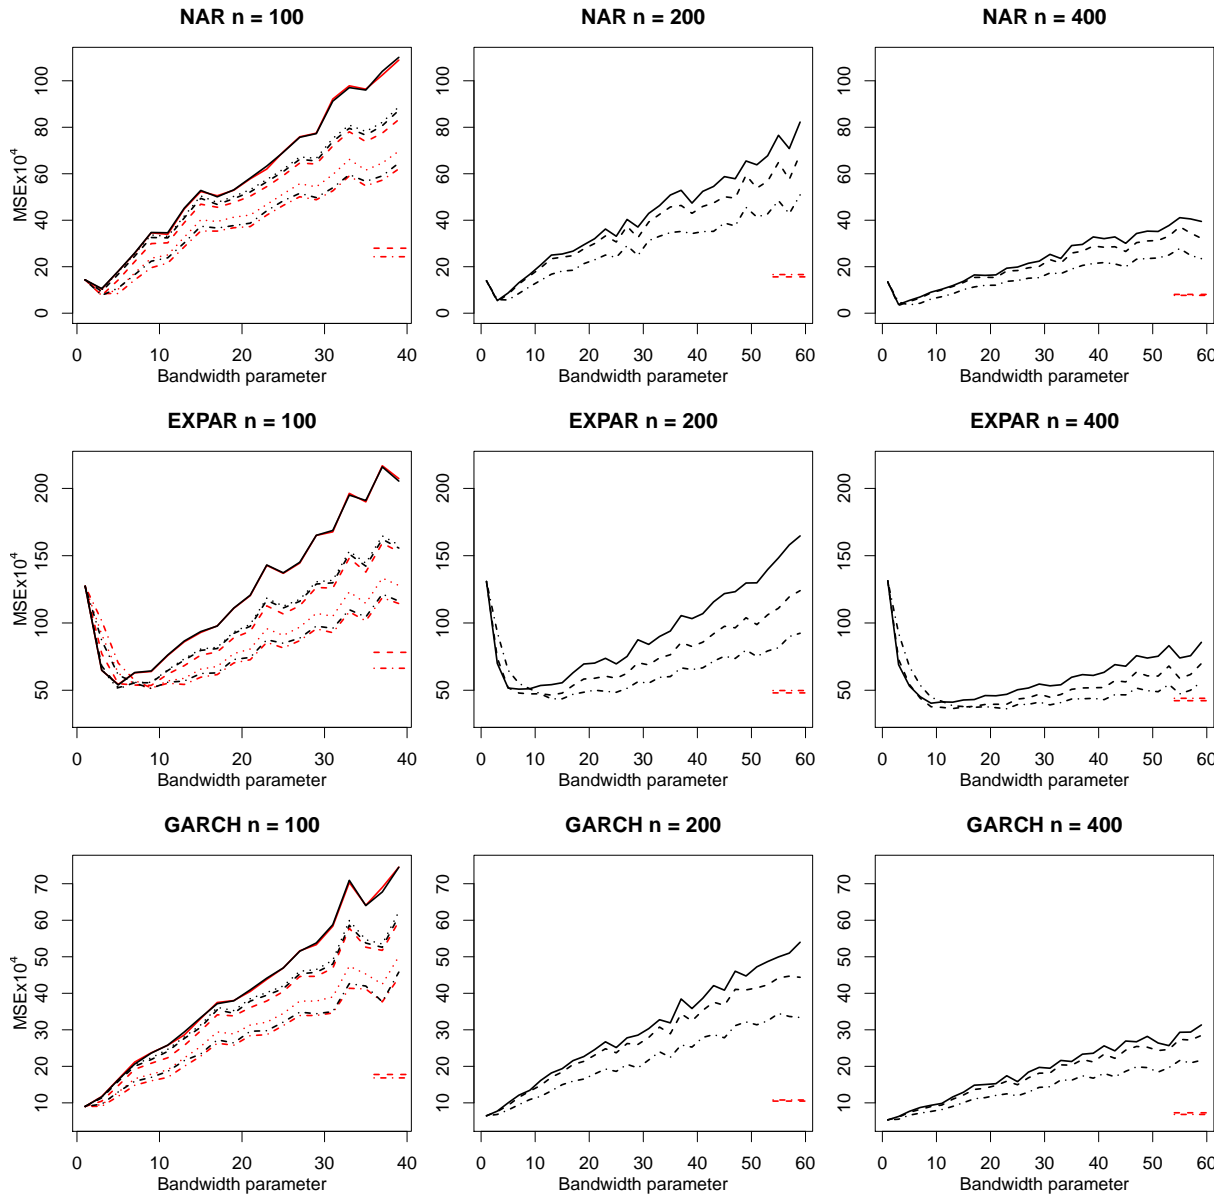

## G.2.5 Statistic $T_n$ , $p = 0.95$

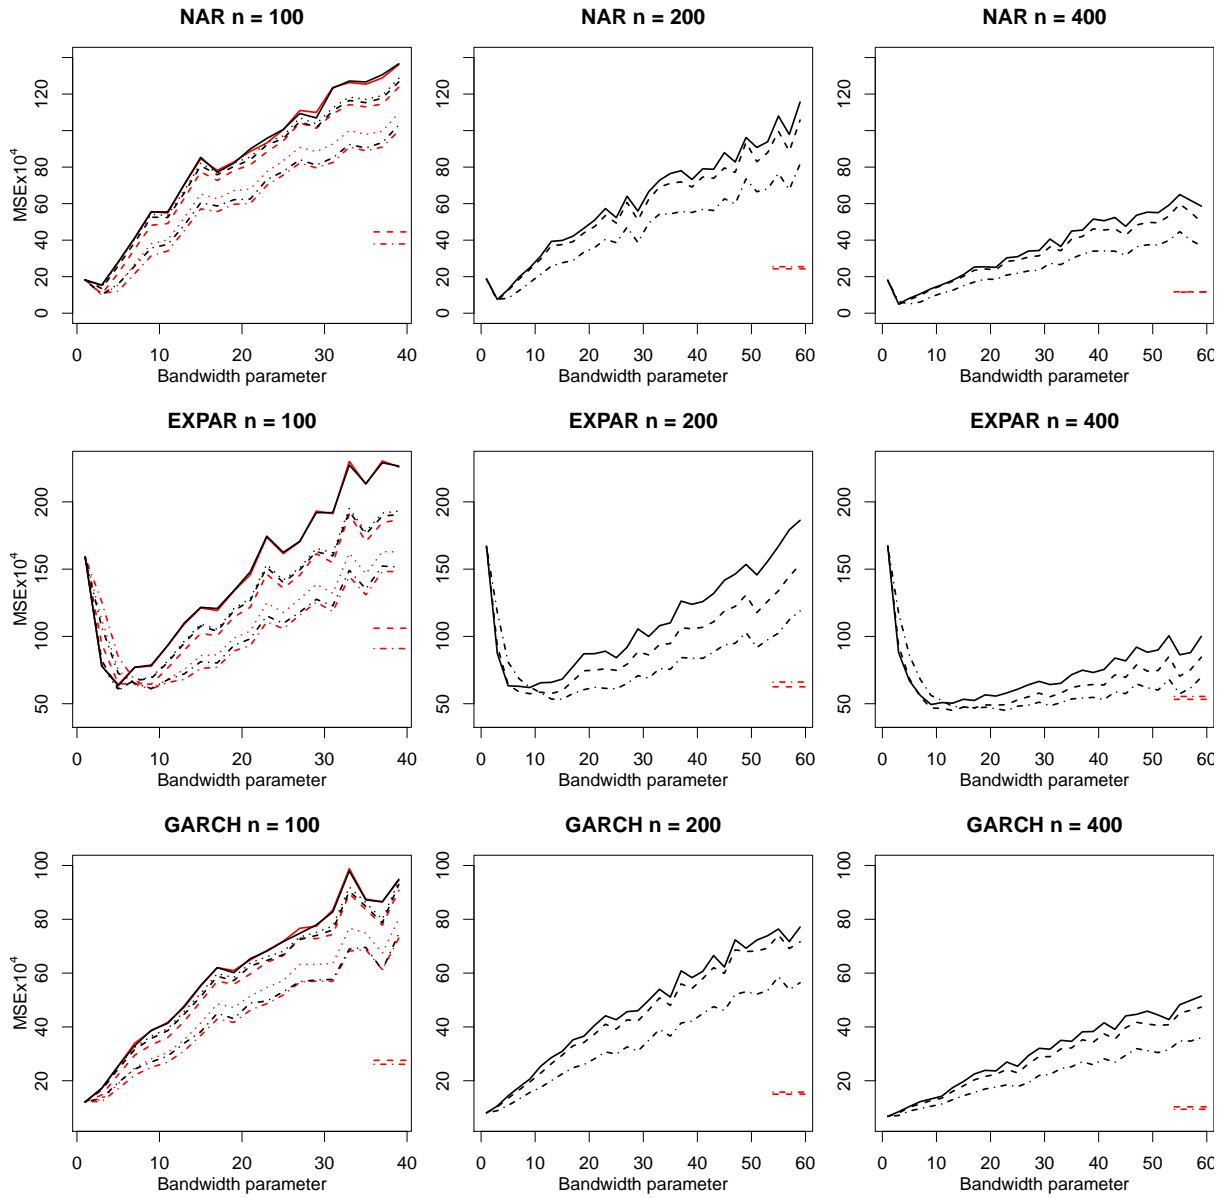

### G.2.6 Statistic $T_n$ , $p = 0.99$

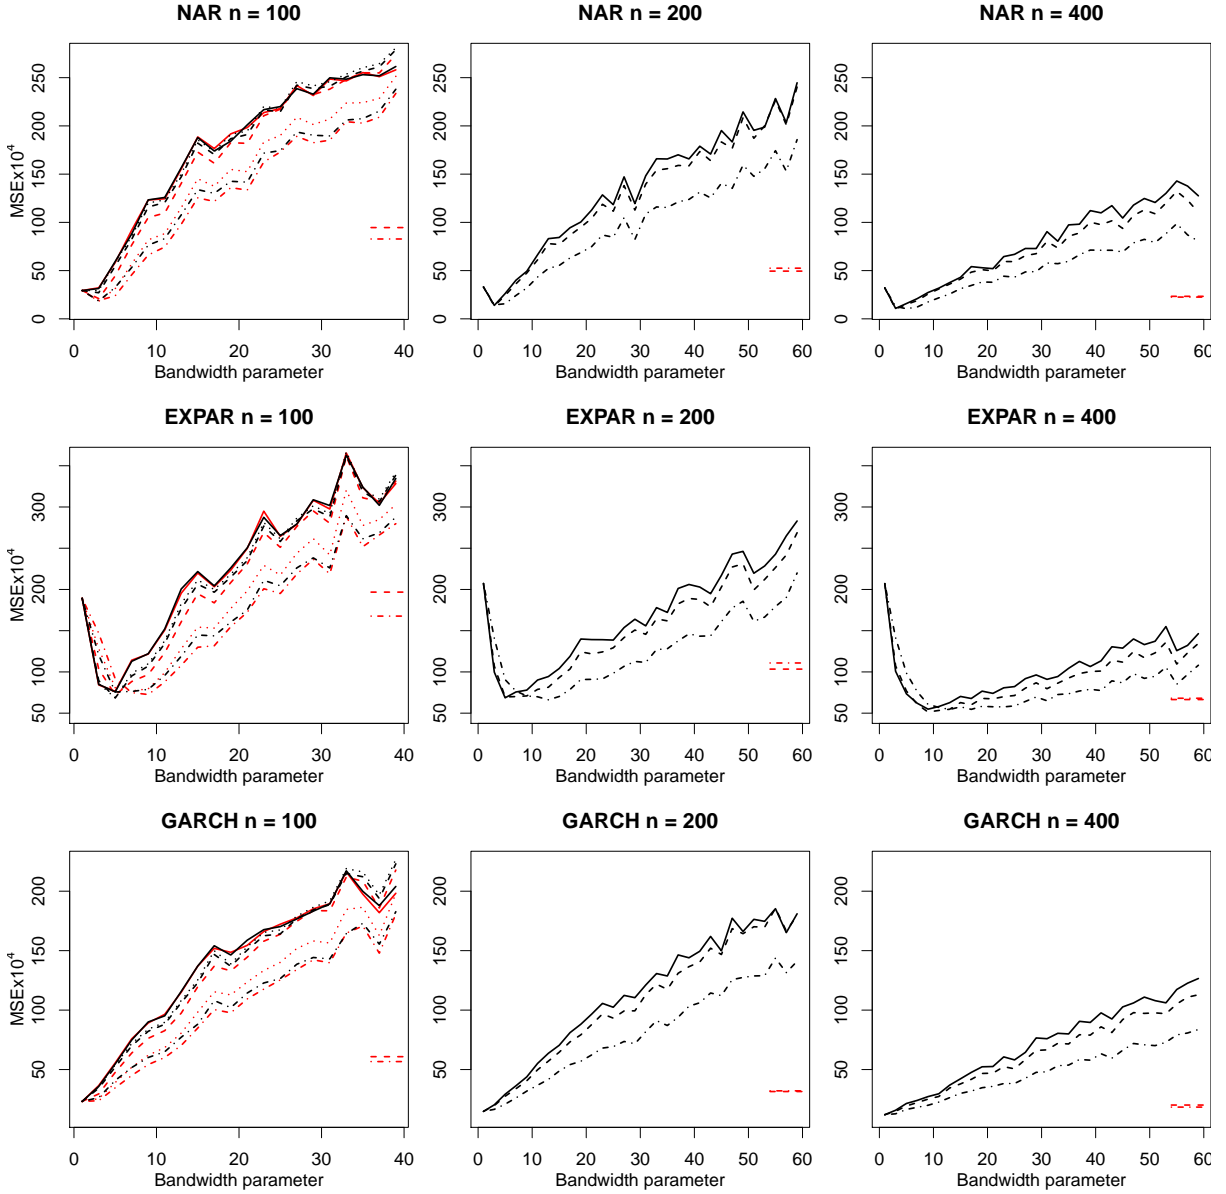

### G.3 Analogues of Figure 2 for simpler statistics

This subsection contains results on the pointwise accuracy of the bootstrap procedure. More precisely, we provide results on the performance of simple bootstrap estimators for quantiles of the statistic  $\mathbb{C}_n(0, 1, \mathbf{u}) = \sqrt{n}\{C_{1:n}(\mathbf{u}) - C(\mathbf{u})\}$  for a fixed  $\mathbf{u} \in [0, 1]^d$ . We proceed as follows. First, since the weak limit  $\mathbb{H}(\mathbf{u}) = \mathbb{C}(0, 1, \mathbf{u})$  is symmetrically distributed around 0, we know that its  $(1 - \alpha)$ -quantile, denoted by  $q_{1-\alpha}$ , satisfies  $q_{1-\alpha} = -q_\alpha$ . Moreover, since

$$\mathbb{P}\{\mathbb{H}(\mathbf{u}) > q_{1-\alpha}\} = \frac{1}{2} \left[ \mathbb{P}\{\mathbb{H}(\mathbf{u}) > q_{1-\alpha}\} + \mathbb{P}\{\mathbb{H}(\mathbf{u}) < -q_{1-\alpha}\} \right] = \frac{1}{2} \mathbb{P}\{|\mathbb{H}(\mathbf{u})| > q_{1-\alpha}\},$$

$q_{1-\alpha}$  is equal to the  $(1 - 2\alpha)$ -quantile of  $|\mathbb{H}(\mathbf{u})| = |\mathbb{C}(0, 1, \mathbf{u})|$ . We approximate the latter by the  $\lfloor n(1 - 2\alpha) \rfloor$ -order statistic of  $|\mathbb{C}_n^{(1)}(0, 1, \mathbf{u})|, \dots, |\mathbb{C}_n^{(M)}(0, 1, \mathbf{u})|$ . Analogues of Figure 2 corresponding to the above setting are given in Subsections G.3.1–G.3.5 below. Additional simulation results which we do not report here for the sake of brevity reveal that this approach seems to result in a smaller MSE than if  $q_{1-\alpha}$  is estimated by the  $\lfloor n(1 - \alpha) \rfloor$ -order statistic of  $\mathbb{C}_n^{(1)}(0, 1, \mathbf{u}), \dots, \mathbb{C}_n^{(M)}(0, 1, \mathbf{u})$ .

For simplicity, we only report results for the case  $d = 2$ ,  $\mathbf{u} = (1/2, 1/2)$  and  $p = 1 - 2\alpha \in \{0.5, 0.75, 0.9, 0.95, 0.99\}$ ; qualitatively similar results were obtained for other choices of  $\mathbf{u}$ . Note that the choice  $\mathbf{u} = (1/2, 1/2)$  is helpful for the construction of asymptotic confidence intervals for estimators of Blomqvist’s beta, the population version of that coefficient being given by  $\beta = 4C(1/2, 1/2) - 1$  (see e.g. Genest et al., 2013).

Finally, note that  $\mathbb{H}(\mathbf{u}) = \mathbb{C}(0, 1, \mathbf{u})$  is normally distributed, whence, in contrast to the more complicated Cramér–von Mises and Kolmogorov–Smirnov statistics, the quantiles  $q_{1-\alpha}$  could alternatively be approximated by estimating the limiting long-run variance and using standard normal quantiles. Estimating the long-run variance could for instance be accomplished using a computable version of the estimator  $\tilde{\sigma}_n(\mathbf{u}, \mathbf{u})$  given in (5.1) in Section 5.1 of the paper and would additionally require the estimation of the partial derivatives of  $C$ . An alternative approach to estimate the long-run variance consists of using the sample variance of the bootstrap sample  $\mathbb{C}_n^{(1)}(0, 1, \mathbf{u}), \dots, \mathbb{C}_n^{(M)}(0, 1, \mathbf{u})$ . The experiments reported in Figure 3 give indirectly an idea on how the value of  $\ell_n$  typically affects that estimator. Simulation results of a similar nature can be found in Shao (2010).

### G.3.1 Statistic $|\mathbb{C}_n(0, 1, 0.5, 0.5)|$ , $p = 0.5$

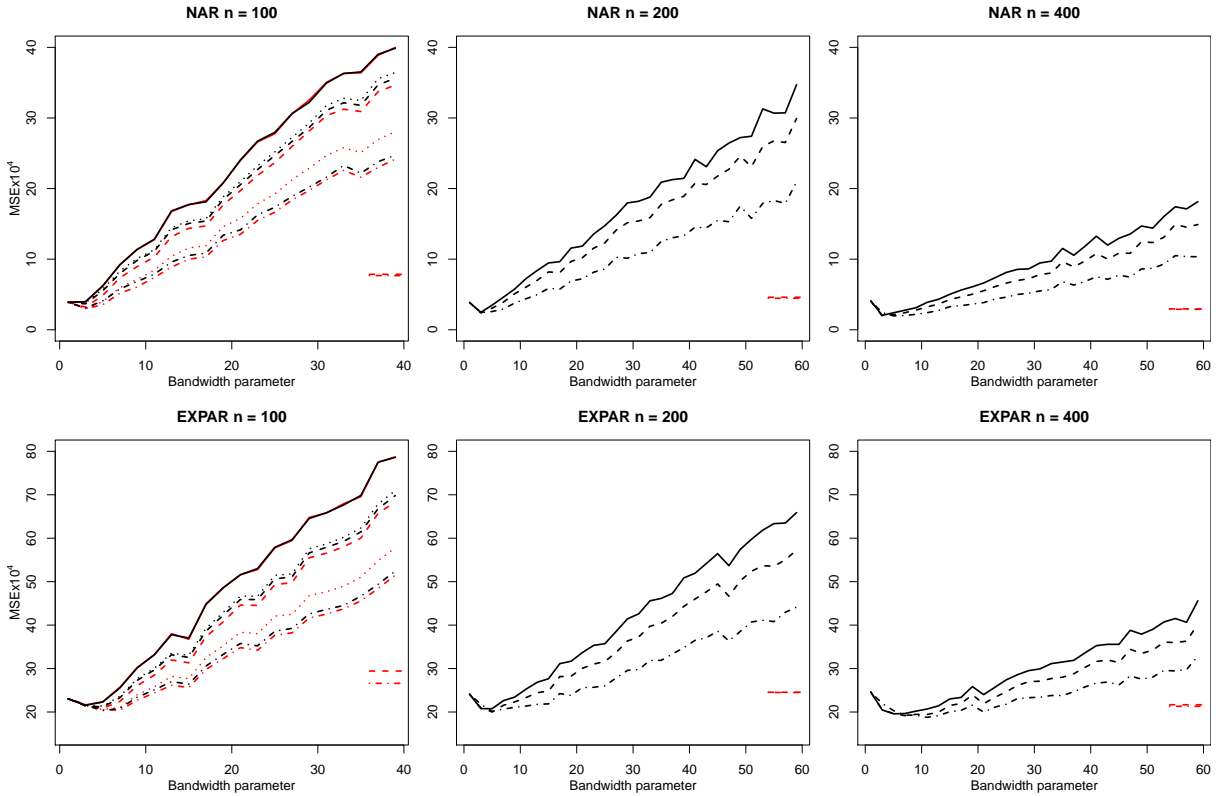

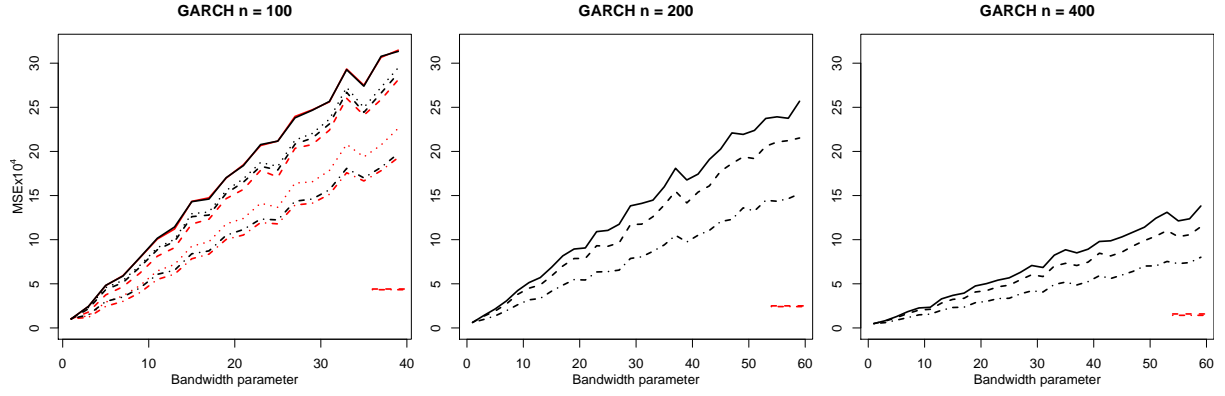

### G.3.2 Statistic $|\mathbb{C}_n(0, 1, 0.5, 0.5)|$ , $p = 0.75$

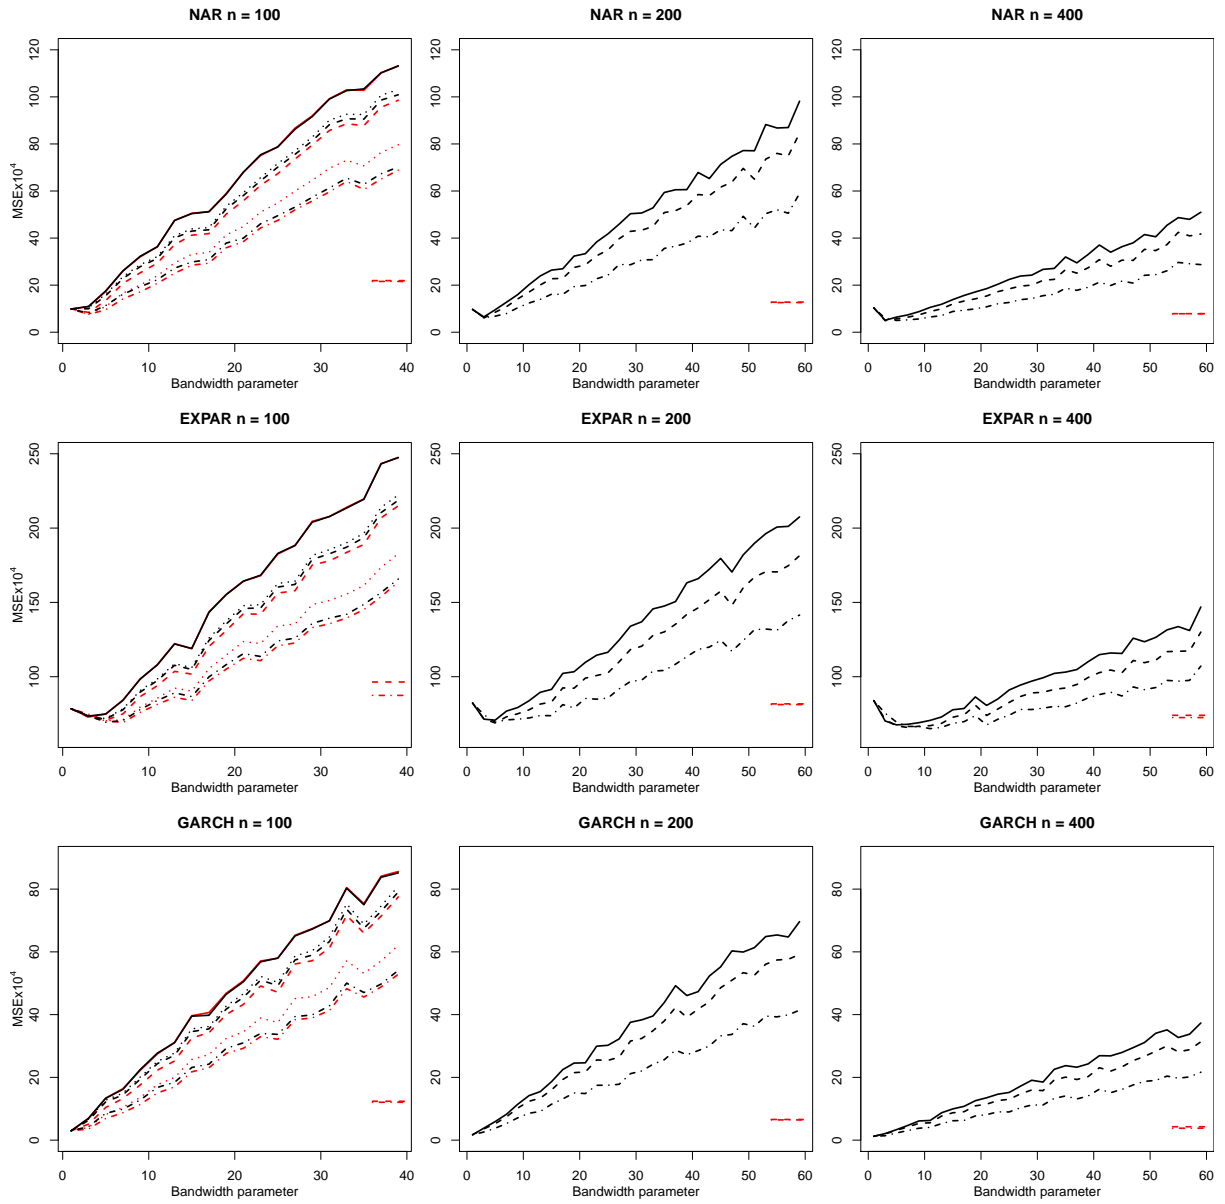

### G.3.3 Statistic $|\mathbb{C}_n(0, 1, 0.5, 0.5)|$ , $p = 0.90$

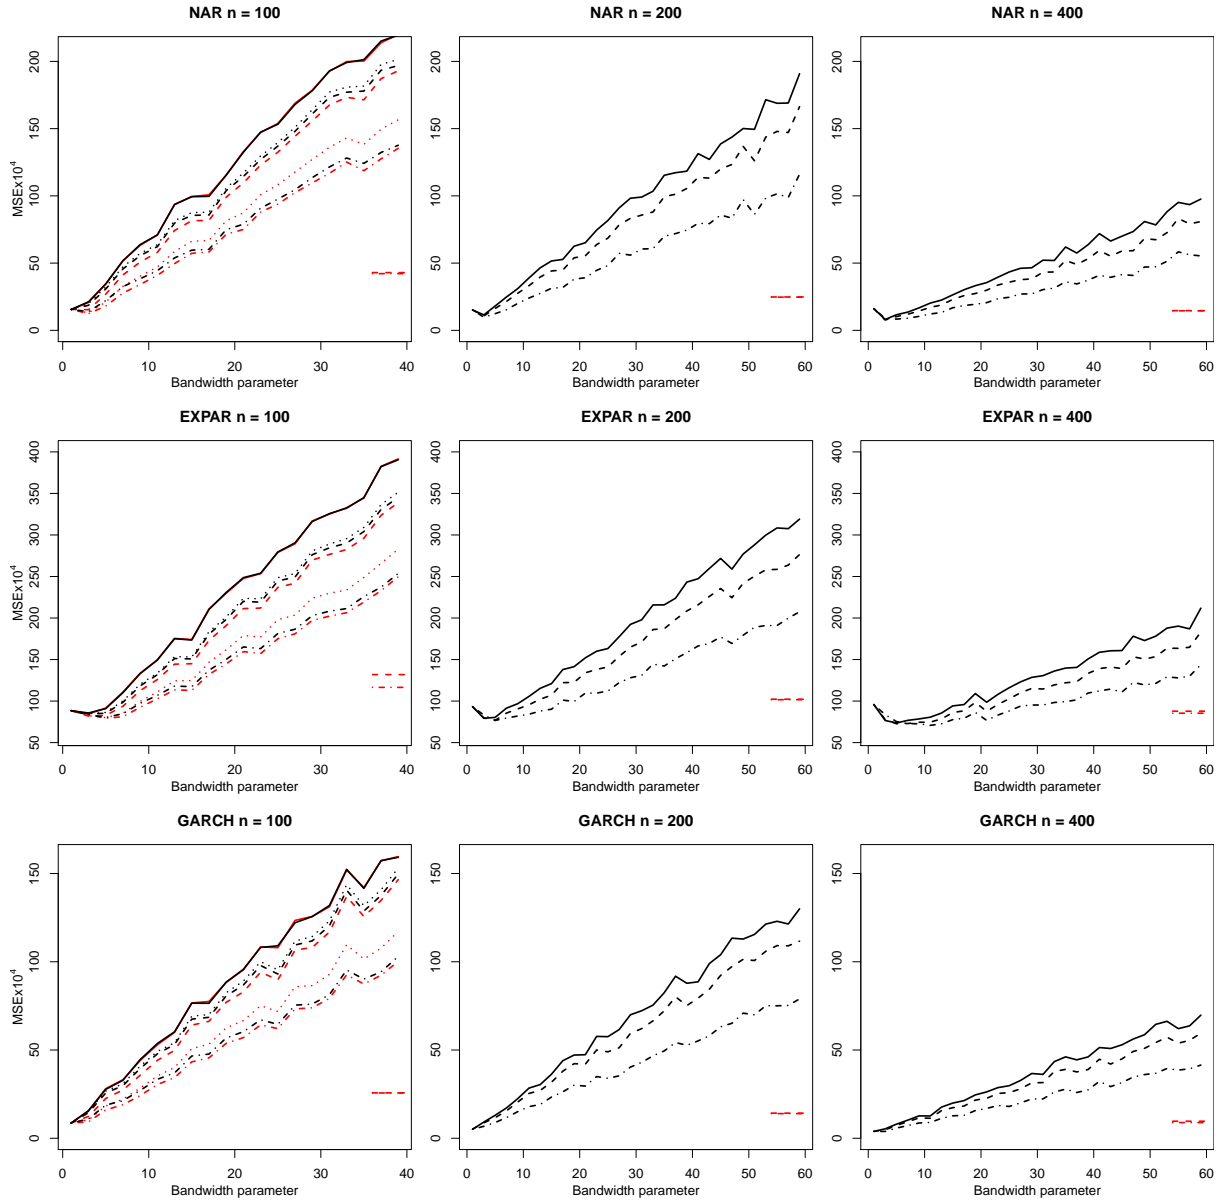

### G.3.4 Statistic $|\mathbb{C}_n(0, 1, 0.5, 0.5)|$ , $p = 0.95$

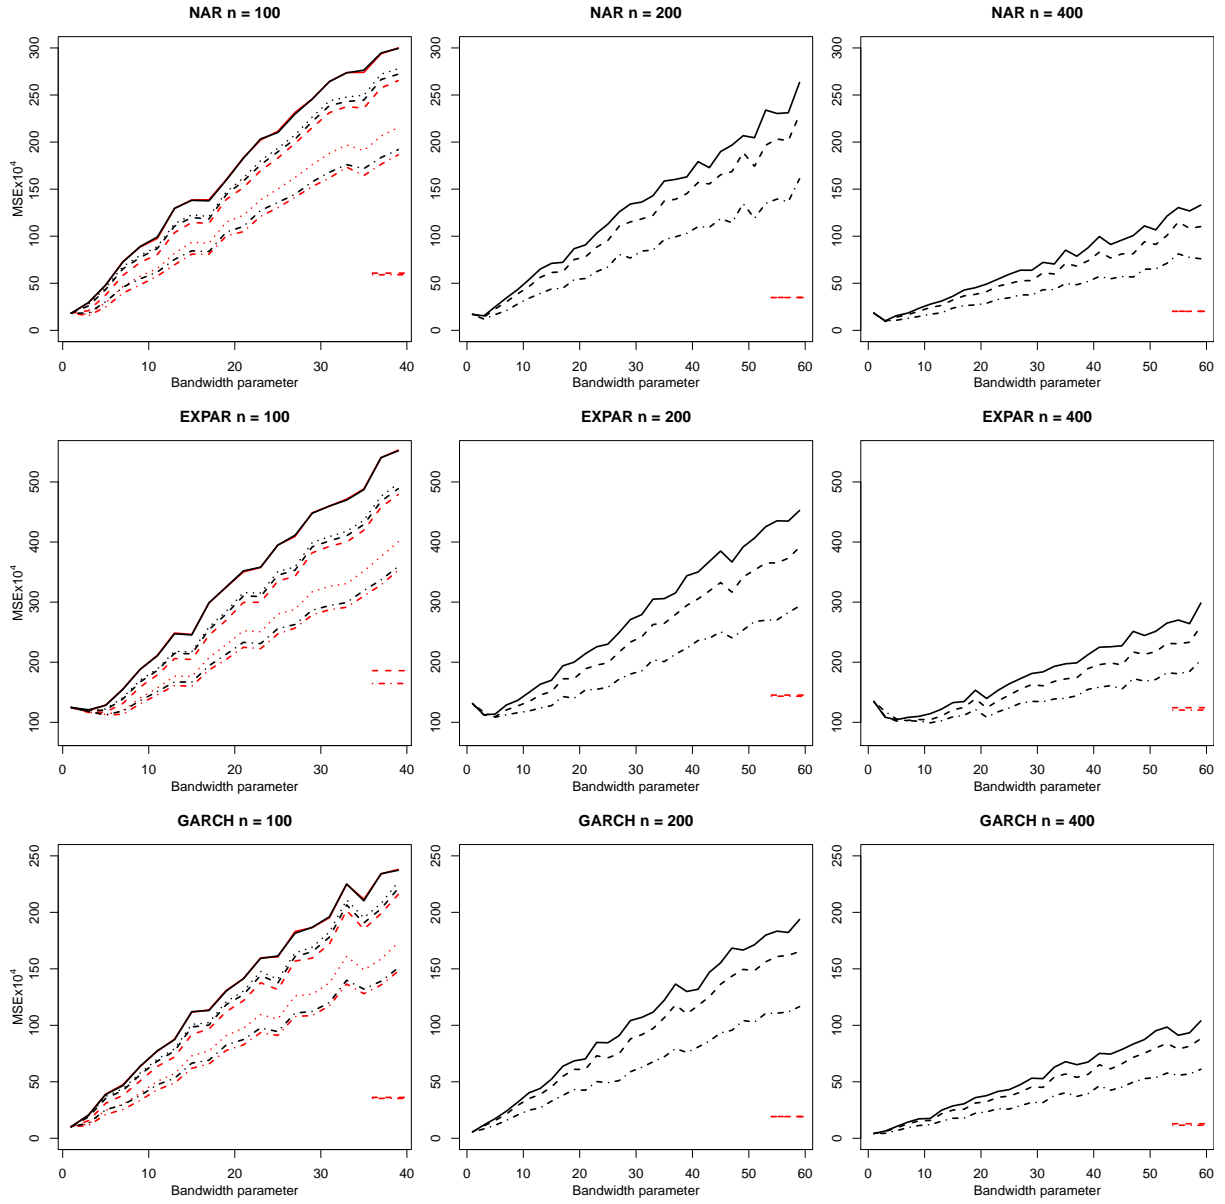

### G.3.5 Statistic $|\mathbb{C}_n(0, 1, 0.5, 0.5)|$ , $p = 0.99$

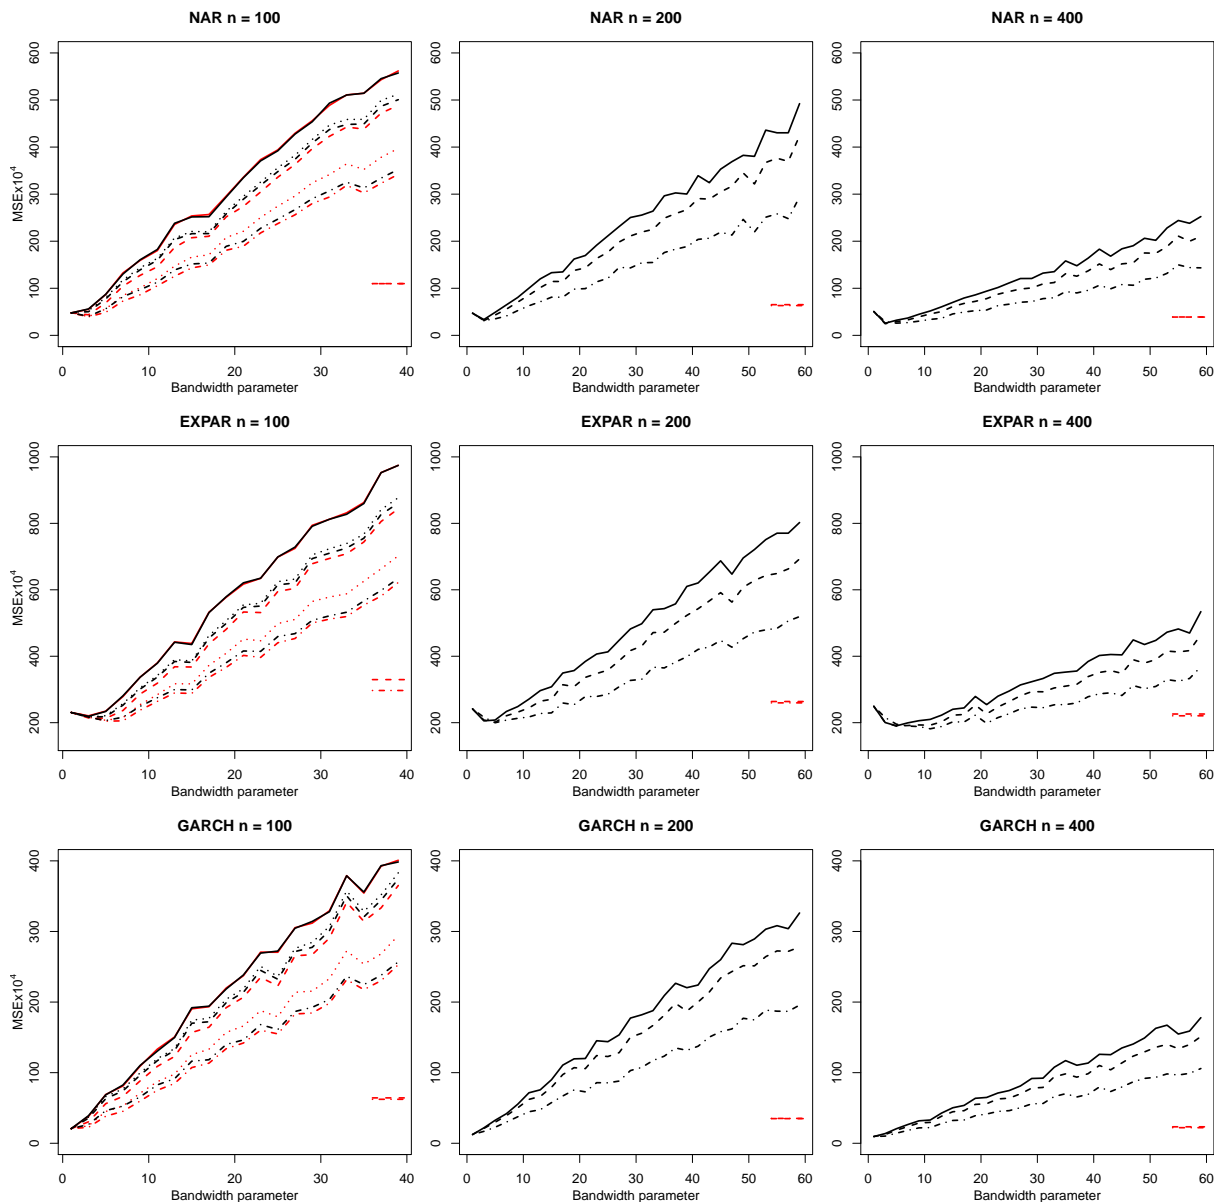

## References

- A. Bücher. A note on weak convergence of the sequential multivariate empirical process under strong mixing. *Journal of Theoretical Probability*, page in press, 2014.
- A. Bücher, S. Jäschke, and D. Wied. Nonparametric tests for constant tail dependence with an application to energy and finance. *Available at SSRN*, 2014. URL <http://dx.doi.org/10.2139/ssrn.2422386>.
- H. Dehling and W. Philipp. Empirical process techniques for dependent data. In

- H. Dehling, T. Mikosch, and M. Sorensen, editors, *Empirical process techniques for dependent data*, pages 1–113. Birkhäuser, Boston, 2002.
- C. Genest, A. Carabarin-Aguirre, and F. Harvey. Copula parameter estimation using blomqvist’s beta. *Journal de la Société Française de Statistique*, 154(1):5–24, 2013.
- H.R. Künsch. The jackknife and the bootstrap for general stationary observations. *Annals of Statistics*, 17(3):1217–1241, 1989.
- J. Segers. Asymptotics of empirical copula processes under nonrestrictive smoothness assumptions. *Bernoulli*, 18:764–782, 2012.
- X. Shao. The dependent wild bootstrap. *Journal of the American Statistical Association*, 105(489):218–235, 2010.
- A.W. van der Vaart. *Asymptotic statistics*. Cambridge University Press, 1998.
